# Supplementary material for: The effect of the A-site cation on the phase transition temperature of metal halide perovskites
Source: arXiv:2602.20058 source file (2026-02-23)
Supplement: Supplementary file 1 [file si.pdf]

# The effect of the A-site cation on the phase transition temperature of metal halide perovskites

Tom Braeckevelt,[†] [‡]Sander Vandenhaute,[†] Sven M. J. Rogge,[†] Johan Hofkens,[‡] and Veronique Van Speybroeck[*,†]

[†]*Center for Molecular Modeling (CMM), Ghent University, Technologiepark-Zwijnaarde 46, 9052 Zwijnaarde, Belgium, and*

[‡]*Department of Chemistry, KU Leuven, Celestijnenlaan 200F, Leuven 3001, Belgium*

E-mail: Veronique.VanSpeybroeck@UGent.be

[†]Ghent University
[‡]KU Leuven Chemistry

# Table of contents


**1 Quantum versus classical description of the nuclei** **S-3**

**2 VASP settings for the benchmark of the exchange correlation functionals** **S-5**

2.1 Convergence PBE+D3(BJ) forces . . . . . . . . . . . . . . . . . . . . . . . . . . . . . . . . S-5

2.2 Convergence RPA+HF forces . . . . . . . . . . . . . . . . . . . . . . . . . . . . . . . . . . S-7

**3 Bias potential for organic molecules** **S-9**

3.1 Formamidinium . . . . . . . . . . . . . . . . . . . . . . . . . . . . . . . . . . . . . . . . S-10

3.2 Methylammonium . . . . . . . . . . . . . . . . . . . . . . . . . . . . . . . . . . . . . . . S-10

**4 Level of theory effect on the ground state energies** **S-12**

**5 Analysis of the free energy contributions** **S-15**

5.1 Finding the ground state structure and frequencies . . . . . . . . . . . . . . . . . . . . . . S-15

5.2 Going from the harmonic to the intermediate PES . . . . . . . . . . . . . . . . . . . . . . S-17

5.3 Temperature correction to the Helmholtz free energy for the intermediate PES . . . . . . . . S-18

5.4 Going from the intermediate to the MLP PES . . . . . . . . . . . . . . . . . . . . . . . . . S-20

5.5 Temperature correction to the Helmholtz free energy for the MLP PES . . . . . . . . . . . . S-21

5.6 Going from Helmholtz to Gibbs free energy . . . . . . . . . . . . . . . . . . . . . . . . . . S-22

5.7 Temperature correction to the Gibbs free energy for the MLP PES . . . . . . . . . . . . . . S-23

5.8 Spectra from NVE MD simulations . . . . . . . . . . . . . . . . . . . . . . . . . . . . . . . S-24

**6 Parameters of the average cell used to calculate the Helmholtz free energy** **S-26**

**7 Histogram of optimized energies** **S-31**

**8 Supercell effect on the free energy contributions** **S-36**

**9 Orientation of the organic molecules** **S-41**

# 1 Quantum versus classical description of the nuclei

Within the harmonic approximation, we can calculate the correction to the classical free energy, $F_{\text{H, clas}}$, for each mode to obtain the quantum mechanical free energy, $F_{\text{H, qm}}$:[1]

$$\Delta F_{\text{H}}(\nu, T) = F_{\text{H, qm}}(\nu, T) - F_{\text{H, clas}}(\nu, T) = k_{\text{B}} T \ln \left[ \frac{1 - \exp\left(-\frac{h\nu}{k_{\text{B}}T}\right)}{\frac{h\nu}{k_{\text{B}}T} \exp\left(\frac{-h\nu}{2k_{\text{B}}T}\right)} \right], \tag{S1.1}$$

$h$ is the Planck constant, $k_{\text{B}}$ is the Boltzmann constant, $T$ is temperature, and $\nu$ is the frequency of a mode. For a harmonic potential energy surface (PES) the difference between the classical and quantum vibrational free energy becomes negligible at higher temperatures or lower frequencies, as shown on the left side of Fig. S1.

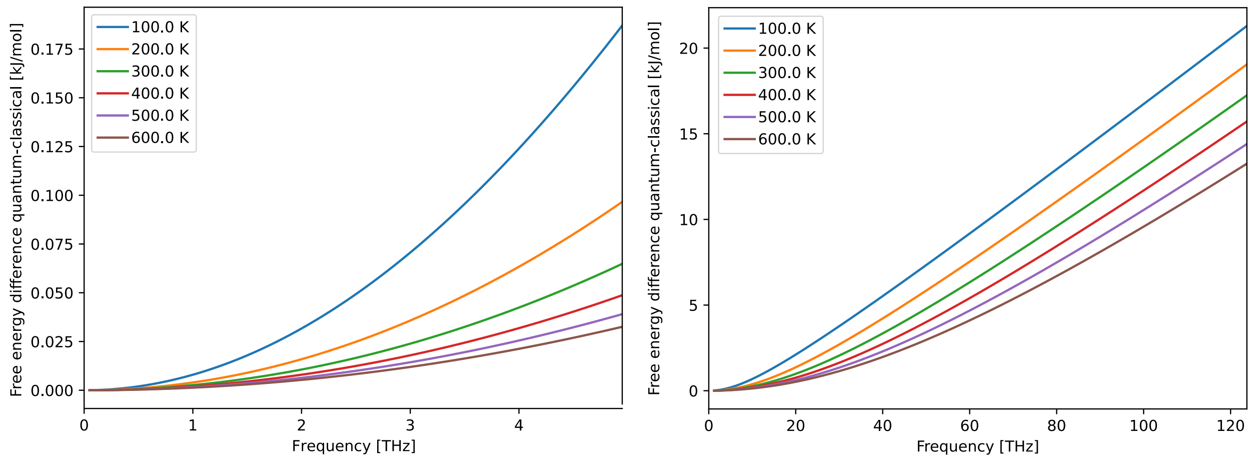


Figure S1: Vibrational free energy difference per mode between a classical and quantum description of the nuclei as a function of the frequency and temperature. The left figure provides a zoomed-in picture of the right figure, to indicate that the quantum free energy difference is approximately the same as the classical free energy for low frequencies and high temperatures.

Heavy nuclei lead to low frequencies and therefore a classical description is sufficient. For the organic molecules a quantum description is necessary. However, the terms in the thermodynamic integration (TI) procedure discussed in Sec. 2 of the main text, assume a classical description of the nuclei. As explained by Kapil and coworkers, it is possible to perform a thermodynamic integration correction to go from the classical to the quantum free energy by applying path integral MD calculations.[2] This is outside the scope of the current paper.

If we sum (or integrate) over all frequencies and subtract the free energy correction for the $\delta$

phases with the correction of the $\gamma$ phase, we find the temperature-dependent correction for the free energy differences, the results for $CsPbI_3$, $FAPbI_3$, and $MAPbI_3$ are reported in Tab. S1.

Table S1: Correction to Helmholtz free energy which is the difference between the quantum mechanical free energy and the classical free energy. The correction is obtained via the harmonic approximation, see Eq. S1.1. The differences between the $\delta$ phases and the $\gamma$ phase are reported for the three investigated materials in kJ/mol per formula unit (pfu). For each material three different unit cells are investigated, namely the average unit cell during a NPT MD simulation at 0.1 MPa and at 234, 350, or 501 K.

| $F_{H,qm} - F_{H,clas}$ | $\delta_{Cs} - \gamma$ | | | $\delta_{FA} - \gamma$ | | |
|---|---|---|---|---|---|---|
| pfu [kj/mol] | **h**(T=234 K) | **h**(T=350 K) | **h**(T=501 K) | **h**(T=234 K) | **h**(T=350 K) | **h**(T=501 K) |
| $CsPbI_3$ | 0.02 | 0.02 | 0.02 | 0.01 | 0.02 | 0.02 |
| $FAPbI_3$ | -0.54 | -0.62 | -0.64 | 0.20 | -0.31 | -0.27 |
| $MAPbI_3$ | -0.29 | -0.35 | -0.40 | 022 | 0.18 | 0.06 |

Because $CsPbI_3$ only has heavy nuclei, the frequencies are low, and the correction is small. This correction is larger for $FAPbI_3$, and $MAPbI_3$ due to the organic molecules. However, the correction remains small because the high-frequency modes are similar for all three phases.

## 2 VASP settings for the benchmark of the exchange correlation functionals

To benchmark the energies, the same settings as explained in our previous work were used.[3] Only for the RPA+HF calculations, the precision setting of the fast Fourier transform grids used to calculate the RPA correlation was increased to "Normal", and the kpoint grids were slightly reduced to $3 \times 3 \times 2$, $6 \times 3 \times 1$, and $3 \times 2 \times 3$ grids for the $\gamma$, $\delta_{Cs}$, and $\delta_{FA}$ phases, respectively. Because forces are derivatives of the energy, the convergence could be more problematic. Therefore, convergence tests for the forces were performed, see the next subsections. The same settings as for the energy calculations were used for the force calculations. Only the RPA+HF settings were slightly changed. The cut-off energy for the RPA+HF calculations increased to 600 eV, the precision setting of the fast Fourier transform grids was increased to "Accurate", and the kpoint grids were decreased to $2 \times 2 \times 2$, $4 \times 2 \times 4$, and $2 \times 2 \times 2$ grids for the $\gamma$, $\delta_{Cs}$, and $\delta_{FA}$ phases, respectively.

### 2.1 Convergence PBE+D3(BJ) forces

The convergence of the cut-off energy was determined for a random structure in the $\gamma$ phase containing 4 formula units. The results are depicted in Fig. S2 and Tab. S2. The forces do not change significantly when increasing the cut-off energy beyond 400 eV for $CsPbI_3$. For $FAPbI_3$ the forces converge more slowly and a cut-off energy of 500 eV is necessary. Using a kpoint grid with only 4 kpoints leads to a huge error in the forces of lead and iodine. A kpoint grid of $3 \times 3 \times 2$ is sufficient to get accurate forces. Setting LREAL to Auto also introduces an error, while the other settings have an insignificant effect.

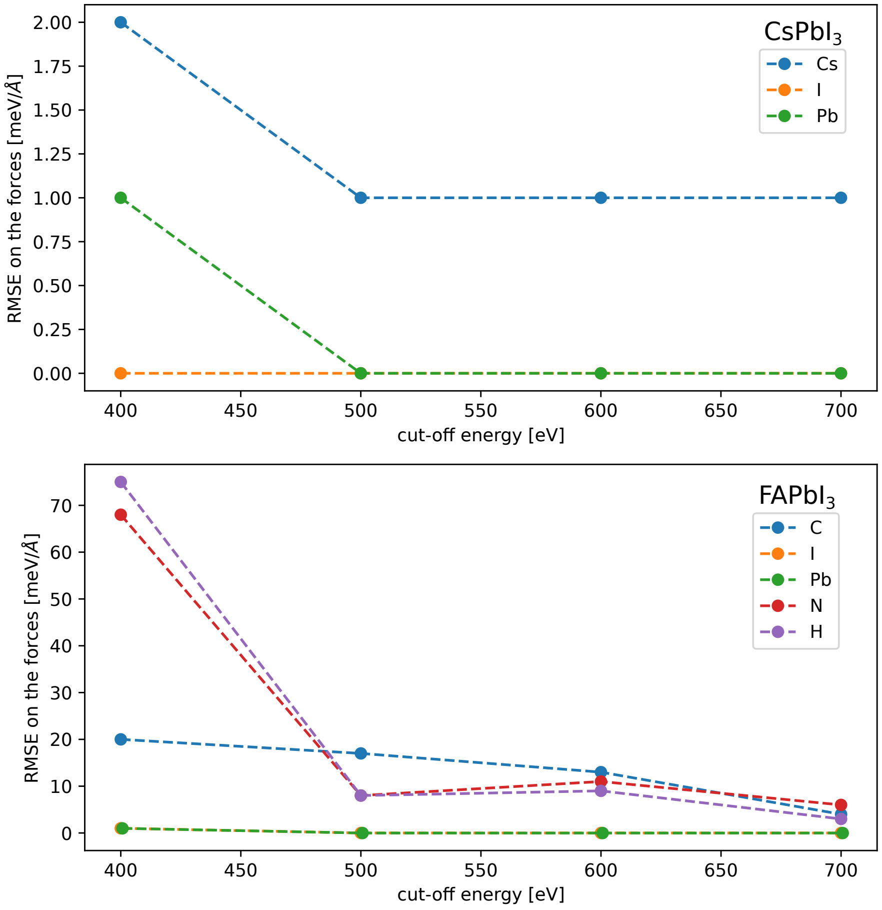


Figure S2: The root mean square error on the PBE+D3(BJ) forces for $CsPb_3$ and $FAPbI_3$ partitioned per element. A random structure of the $\gamma$ phase was used containing 4 formula units. The error was determined with respect to the forces obtained with a cut-off energy of 800 eV.

Table S2: Overview of the effect of the VASP settings on the PBE+D3(BJ) forces for $CsPb_3$ and $FAPbI_3$ partitioned per element. The first column indicates which setting is changed with respect to the reference settings (*i.e.*, kpoints = $4 \times 4 \times 3$, PREC = Accurate, ADDGRID = False, LREAL = False, and EDIFF = $10^{-5}$) while all other settings are kept at their reference value.

| RMSE forces [meV/Å] | $CsPbI_3$ | | | $FAPbI_3$ | | | | |
|---|---|---|---|---|---|---|---|---|
| | Cs | Pb | I | H | C | N | Pb | I |
| kpoints = $2 \times 2 \times 1$ | 12 | 150 | 175 | 8 | 12 | 11 | 138 | 135 |
| kpoints = $3 \times 3 \times 2$ | 1 | 10 | 11 | 0 | 1 | 1 | 7 | 7 |
| kpoints = $5 \times 5 \times 4$ | 0 | 1 | 1 | 0 | 0 | 0 | 1 | 1 |
| PREC = Normal | 2 | 1 | 0 | 0 | 0 | 1 | 1 | 0 |
| ADDGRID =.TRUE. | 0 | 0 | 0 | 0 | 0 | 0 | 0 | 0 |
| LREAL = Auto | 6 | 5 | 20 | 2 | 2 | 2 | 5 | 17 |
| EDIFF = $10^{-8}$ | 1 | 1 | 1 | 0 | 1 | 1 | 0 | 0 |

## 2.2 Convergence RPA+HF forces

The convergence of the cut-off energy was determined for a random structure in the $\gamma$ phase containing 4 formula units. The results are depicted in Fig. S3 and Tab. S3. The root mean square error (RMSE) on the RPA+HF forces is significantly higher than for PBE+D3(BJ) at the same cut-off energy. The RMSE on the forces goes below 50 meV/Å for all elements only at 600 eV. The forces clearly decrease with increasing cut-off energy, only the error for Cs shows an oscillating behavior around a RMSE of 50 meV/Å. The precision setting of the fast Fourier transform grids has a major effect, definitely the grid used to calculate the RPA correlation (PRECFOCK) has to be set to Normal. The kpoint grids can be reduced to $2 \times 2 \times 2$ without significantly changing the forces. Also, the number of frequency points (NOMEGA) has a minor effect.

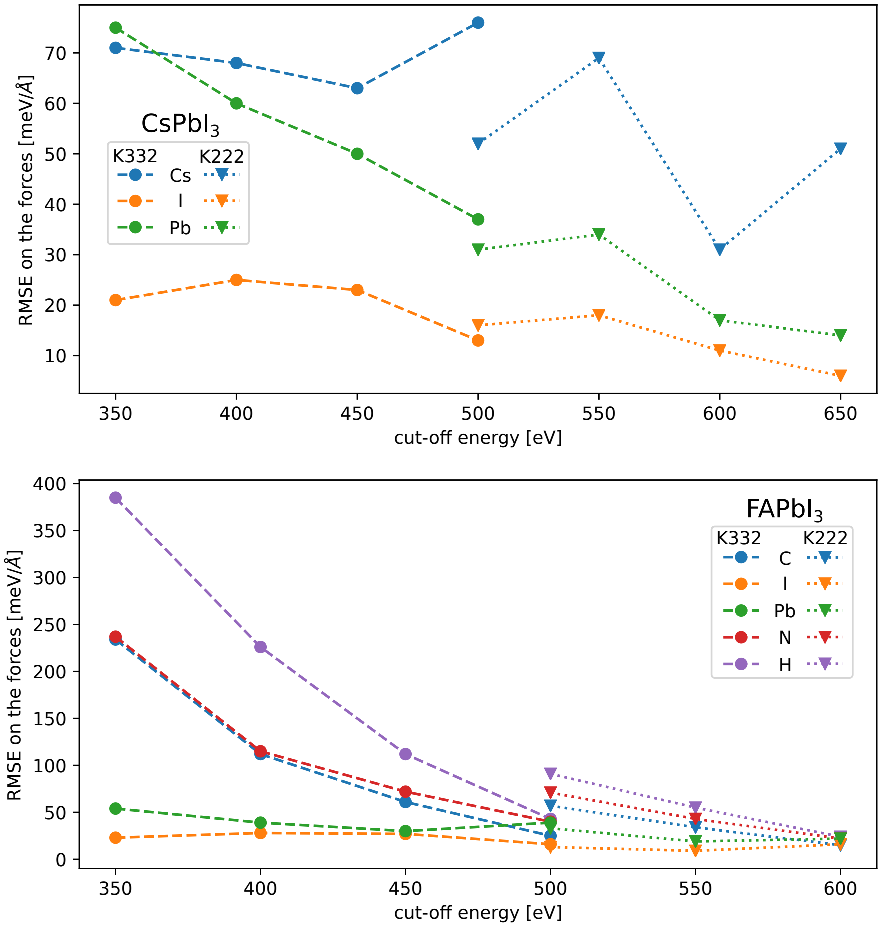


Figure S3: The root mean square error on the RPA+HF forces for $CsPb_3$ and $FAPbI_3$ partitioned per element. A random structure of the $\gamma$ phase was used containing 4 formula units. The error was determined with respect to the forces obtained with a cut-off energy of 550 eV for a $3 \times 3 \times 2$ kpoint grid. For the calculations with a $2 \times 2 \times 2$ kpoint grid, the reference forces were calculated with 700, and 650 eV as cut-off energy for $CsPbI_3$, and $FAPbI_3$, respectively.

Table S3: Overview of the effect of the VASP settings on the RPA+HF forces for $CsPb_3$ and $FAPbI_3$ partitioned per element. The first column indicates which setting is changed with respect to the reference settings (*i.e.*, kpoints = $3 \times 3 \times 2$, PRECFOCK = Normal, PREC = Accurate, and NOMEGA = 8) while all other settings are kept at their reference value.

| RMSE forces [meV/Å] | $CsPbI_3$ | | | $FAPbI_3$ | | | | |
|---|---|---|---|---|---|---|---|---|
| | Cs | Pb | I | H | C | N | Pb | I |
| kpoints = $2 \times 2 \times 2$ | 1 | 5 | 5 | 2 | 1 | 2 | 7 | 7 |
| PRECFOCK = Fast | 115 | 104 | 132 | 590 | 251 | 854 | 242 | 97 |
| PRECFOCK = Accurate | 24 | 21 | 48 | 23 | 7 | 27 | 36 | 22 |
| PREC = Normal | 36 | 24 | 19 | 0 | 2 | 4 | 0 | 0 |
| NOMEGA = 6 | 3 | 2 | 4 | 2 | 3 | 3 | 3 | 2 |
| NOMEGA = 12 | 0 | 0 | 0 | 0 | 1 | 1 | 0 | 0 |

# 3 Bias potential for organic molecules

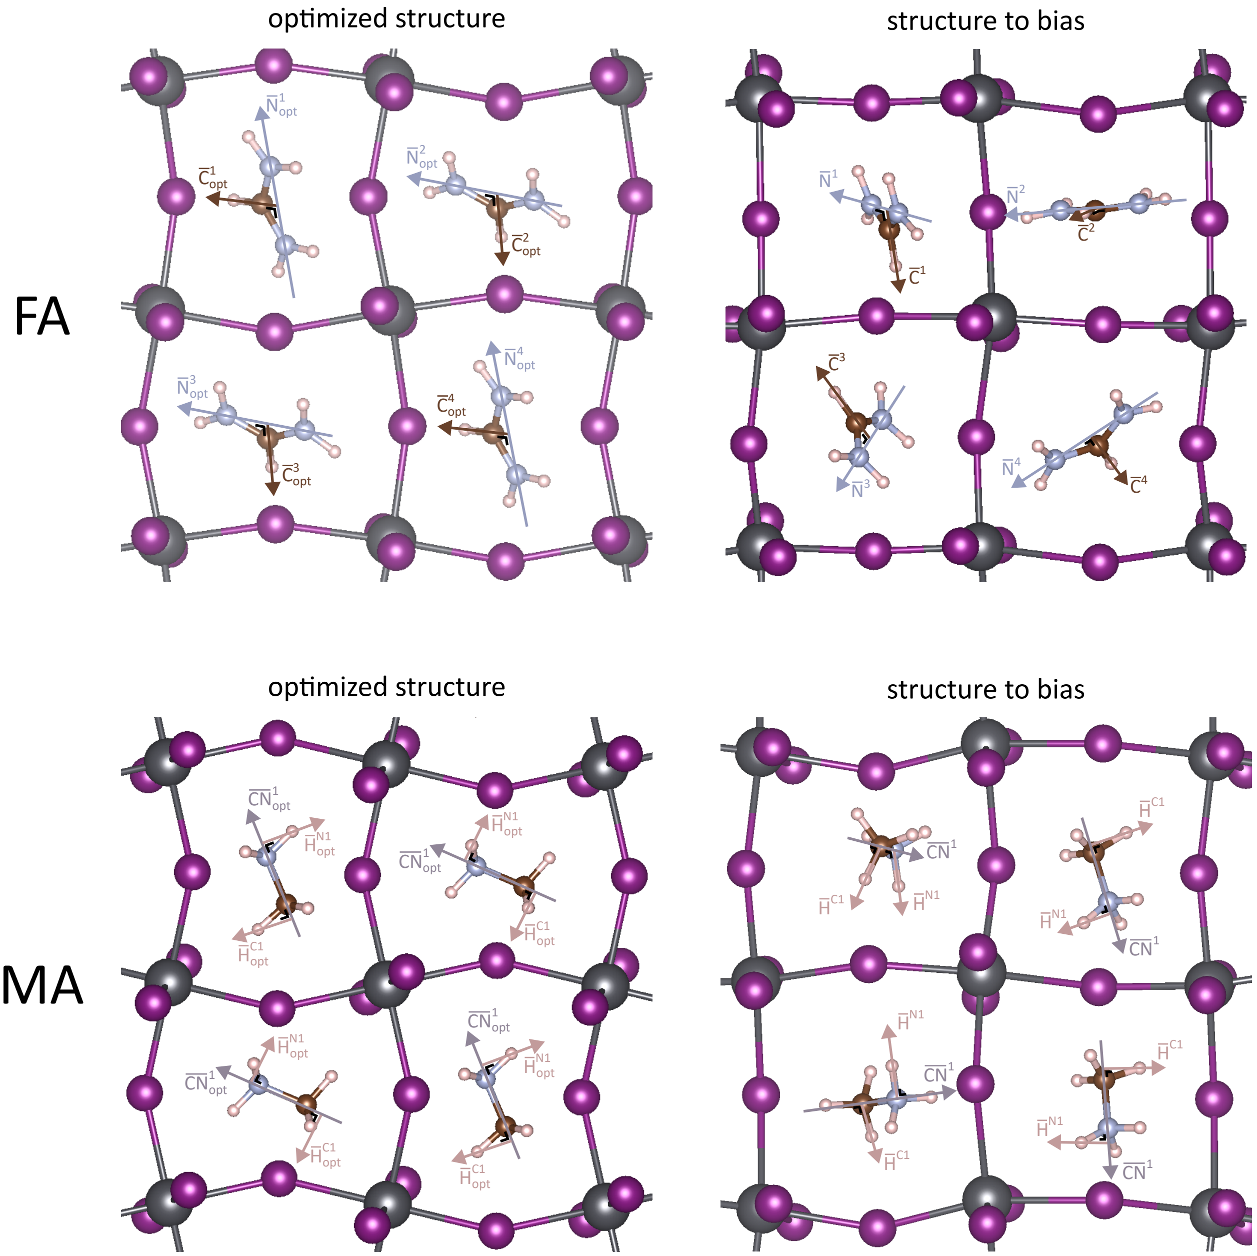


Figure S4: Visual representation of the vectors to define the orientation of the organic FA or MA molecules in the optimized structure and the structure for which the bias will be applied.

W

For the Hessian PES, the organic molecules have a specific orientation. To fix this orientation for the machine learning potential (MLP) PES, we add a bias based on the orientation of the organic molecules with respect to the orientation of the organic molecule in the optimized

structure. The bias is determined for each organic molecule separately. The total bias is the sum of all those biases. For each molecule we define two (for FA) or three (for MA) vectors based on the atomic positions, see Fig. S4. The dot product between the normalized vectors of the optimized structure and the structure for which the bias will be applied, is used as a metric to define the change in orientation. Afterward, a sigmoid function is applied to this dot product. Finally, a harmonic bias is applied when the value of the dot product is lower than 0.95. The exact mathematical values of the bias are provided in the next subsections.

### 3.1 Formamidinium

$$CV^i_{\mathrm{N}} = \frac{1}{1 + \exp\left[5\left(\frac{\vec{N}^i_{\mathrm{opt}}.\vec{N}^i}{|\vec{N}^i_{\mathrm{opt}}||\vec{N}^i|} - 0.95\right)\right]} \tag{S3.1}$$

$$CV^i_{\mathrm{C}} = \frac{1}{1 + \exp\left[5\left(\frac{\vec{C}^i_{\mathrm{opt}}.\vec{C}^i}{|\vec{C}^i_{\mathrm{opt}}||\vec{C}^i|} - 0.95\right)\right]} \tag{S3.2}$$

$$b^i_{\mathrm{N}} = \begin{cases} 800\left(CV^i_{\mathrm{N}}\right)^2 \text{ [kJ/mol]} & \text{if } CV^i_{\mathrm{N}} < 0.95, \\ 0 & \text{if } CV^i_{\mathrm{N}} \geq 0.95. \end{cases} \tag{S3.3}$$

$$b^i_{\mathrm{C}} = \begin{cases} 200\left(CV^i_{\mathrm{C}}\right)^2 \text{ [kJ/mol]} & \text{if } CV^i_{\mathrm{C}} < 0.95, \\ 0 & \text{if } CV^i_{\mathrm{C}} \geq 0.95. \end{cases} \tag{S3.4}$$

The total bias is equal to the sum of all biases, *i.e.* bias $= \Sigma_i^{\text{\#f.u.}} \left(b^i_{\mathrm{N}} + b^i_{\mathrm{C}}\right)$

### 3.2 Methylammonium

$$CV^i_{\mathrm{CN}} = \frac{1}{1 + \exp\left[5\left(\frac{\overrightarrow{CN}^i_{\mathrm{opt}}.\overrightarrow{CN}^i}{\left|\overrightarrow{CN}^i_{\mathrm{opt}}\right|\left|\overrightarrow{CN}^i\right|} - 0.95\right)\right]} \tag{S3.5}$$

$$CV^i_{\mathrm{H}} = \frac{1}{1 + \exp\left[5\left(0.5\frac{\vec{H}^{Ni}_{\mathrm{opt}}.\vec{H}^{Ni}}{|\vec{H}^{Ni}_{\mathrm{opt}}||\vec{H}^{Ni}|} + 0.5\frac{\vec{H}^{Ci}_{\mathrm{opt}}.\vec{H}^{Ci}}{|\vec{H}^{Ci}_{\mathrm{opt}}||\vec{H}^{Ci}|} - 0.95\right)\right]} \tag{S3.6}$$

$$b^i_{\mathrm{N}} = \begin{cases} 800\left(CV^i_{\mathrm{CN}}\right)^2 \text{ [kJ/mol]} & \text{if } CV^i_{\mathrm{CN}} < 0.95, \\ 0 & \text{if } CV^i_{\mathrm{CN}} \geq 0.95. \end{cases} \tag{S3.7}$$

$$b_{\mathrm{H}}^{i} = \begin{cases} 200\left(CV_{\mathrm{H}}^{i}\right)^{2} [\mathrm{kJ/mol}] & \text{if } CV_{\mathrm{H}}^{i} < 0.95, \\ 0 & \text{if } CV_{\mathrm{H}}^{i} \geq 0.95. \end{cases} \tag{S3.8}$$

The total bias is equal to the sum of all biases, *i.e.* bias $= \Sigma_{i}^{\#\mathrm{f.u.}}\left(b_{\mathrm{CN}}^{i} + b_{\mathrm{H}}^{i}\right)$

## 4 Level of theory effect on the ground state energies

In our previous work,[3] we benchmarked exchange-correlation (XC) functionals on optimized structures containing four formula units of $CsPbI_3$, also optimizing the cell degrees of freedom. Here, we extend this benchmark to $FAPbI_3$ and $MAPbI_3$, with results shown in Fig. S5. As discussed in Sec. 7, the rotational freedom of organic molecules introduces numerous local minima. For each phase and material, we optimized ten structures generated from NPT MD simulations at 600 K and 0.1 MPa, all of which relaxed into distinct configurations.

We find that energy differences between optimized structures of the same phase are largely consistent across most XC functionals and dispersion methods. However, the choice of XC functional and dispersion method significantly impacts energy differences between phases, with PBE+D2 and vdW-DF2 standing out as clear outliers. Using the lowest RPA+HF energy for each phase, we determine the ground-state energy (GSE) differences. For $FAPbI_3$, the GSE difference is 7.22 kJ/mol pfu between the $\delta_{\mathrm{Cs}}$ and $\gamma$ phases and 5.26 kJ/mol pfu between the $\delta_{\mathrm{FA}}$ and $\gamma$ phases. For $MAPbI_3$, the corresponding GSE differences are 4.82 kJ/mol pfu and 2.96 kJ/mol pfu, respectively.

It is important to note that this simple optimization procedure probably did not identify the lowest-energy structure for each phase. Fig. S6 presents the results of RPA+HF calculations on MLP-optimized structures. The optimized structures containing eight formula units, without optimizing the cell degrees of freedom, were required for the TI methodology, and the full cell optimized structures were obtained similarly. Specifically, 4000 structures were generated via NVT (NPT) MD simulations at 150 K (and 0.1 MPa). To escape local minima, these MD simulations were coupled via replica exchange (REX) with 31 simulations at higher temperatures, reaching a maximum of 600 K. The structure predicted by the MLP to have the lowest energy was selected as the ground-state structure.

Fig. S6 shows that the MLP reproduces PBE+D3(BJ) energies within a margin of 1 kJ/mol pfu. Furthermore, the PBE+D3(BJ) energies are in good agreement with the RPA+HF results, with GSE differences between phases deviating by at most 2 kJ/mol pfu. Finally, comparing the RPA+HF results for the fully optimized structures in Fig. S6 with the RPA+HF energy differences in Fig. S5, we find small discrepancies, up to 2 kJ/mol pfu. This may be due to supercell effects, though

it is more likely a result of the more comprehensive ground state structure search performed for the TI approach.

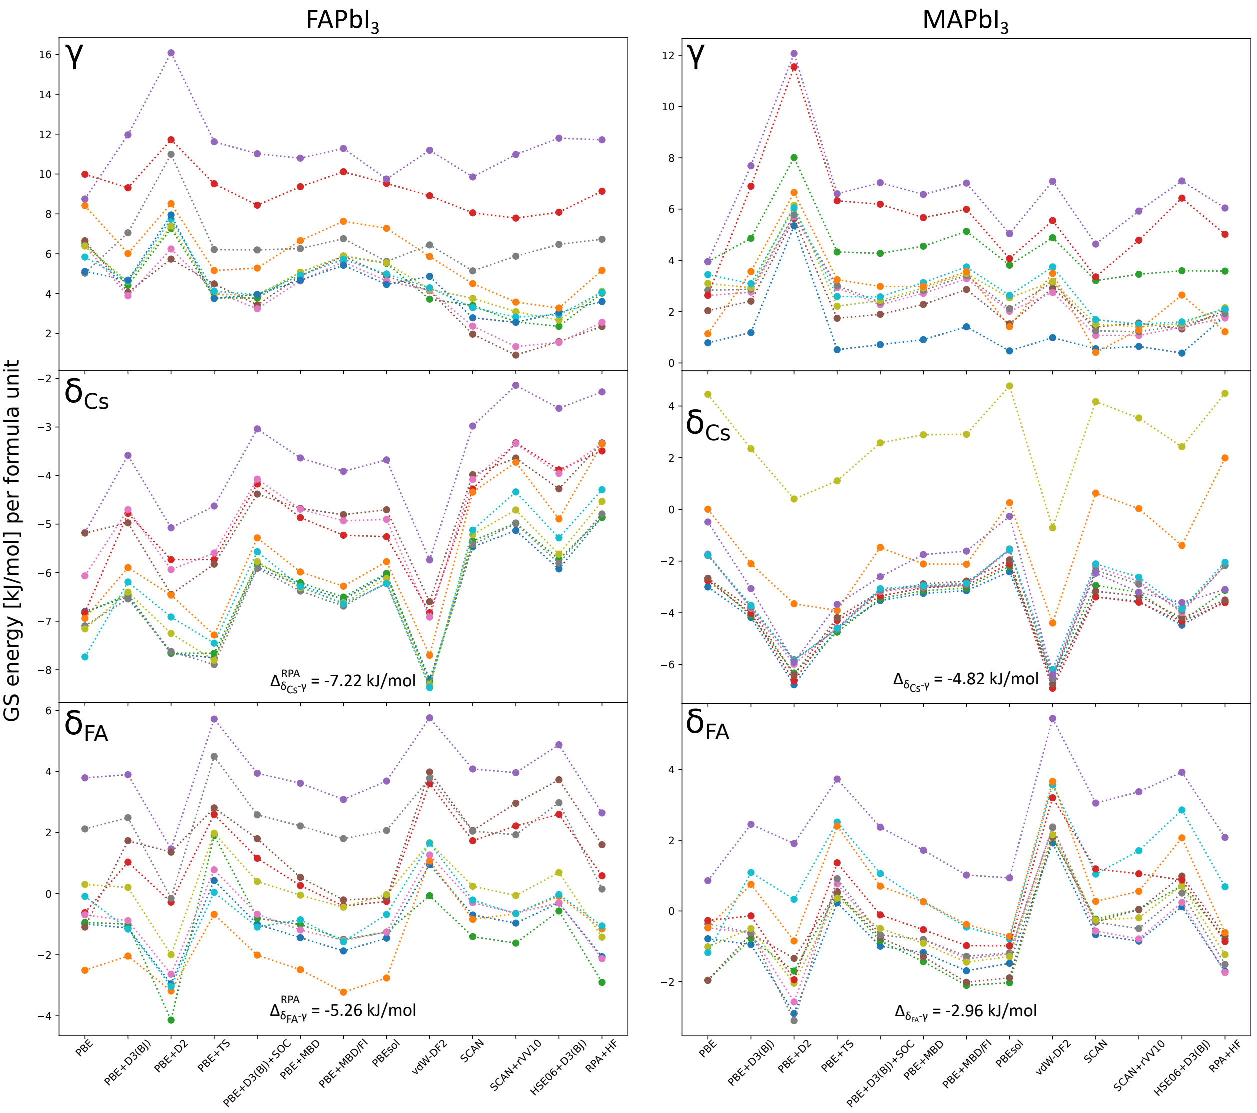


Figure S5: Energy differences between ten NPT optimized structures of the $\gamma$, $\delta_{\text{Cs}}$, and $\delta_{\text{FA}}$ phases for $FAPbI_3$ and $MAPbI_3$, calculated using various methods. The simulations were performed using cells containing four formula units, with structure optimization carried out via density functional theory (DFT) employing the PBE+D3(BJ) exchange-correlation functional.

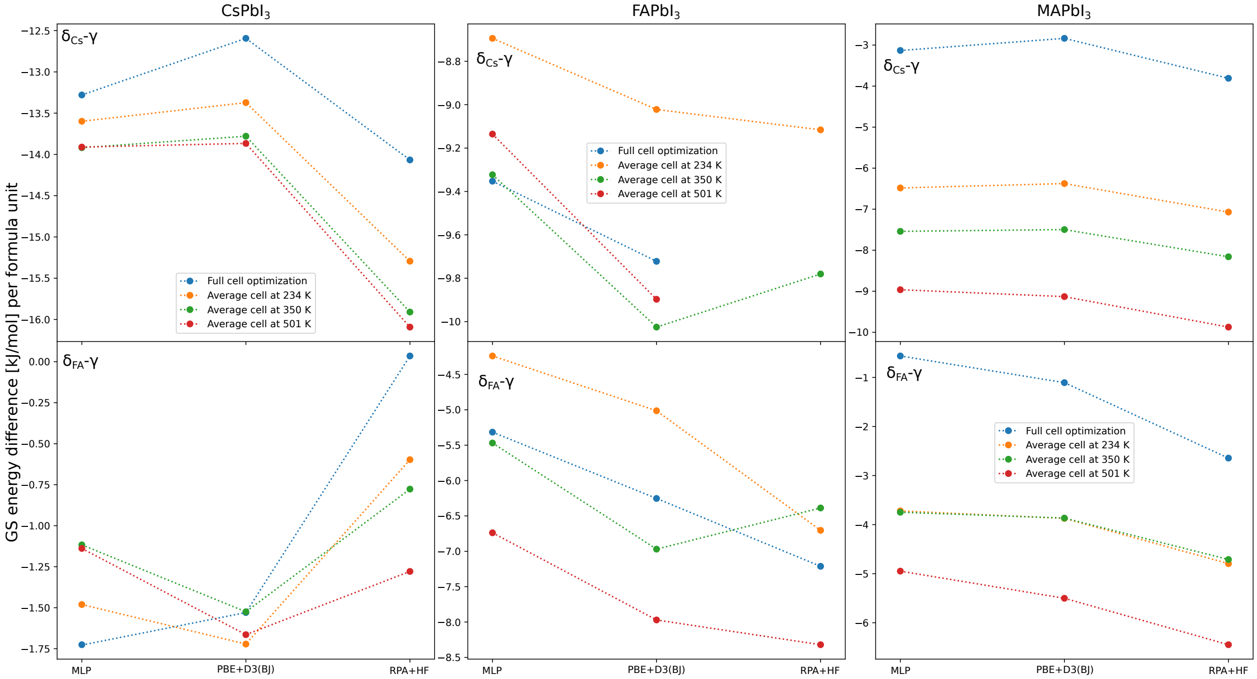


Figure S6: GSE of the $\delta$ phases relative to the $\gamma$ phase for $CsPbI_3$, $FAPbI_3$, and $MAPbI_3$, calculated using MLP, DFT with the PBE+D3(BJ) functional, and RPA+HF. For each phase, structures were optimized using the MLP while keeping the simulation cell containing eight formula units fixed at the average cell dimensions from NPT simulations at 234 K, 350 K, or 501 K. Additionally, a full cell optimization was performed.

# 5 Analysis of the free energy contributions

The complete TI approach requires multiple MD simulations for each structure. The full TI approach can be split into seven contributions for which six contributions require a fixed simulation cell. Each contribution can be analyzed separately. In this section, we will analyze each contribution for the $\gamma$ phase of $FAPbI_3$ using the average cell at 150 K and 0.1 MPa containing eight formula units. The data and plots for all other simulations can be found at https://doi.org/10.5281/zenodo.18108633.

## 5.1 Finding the ground state structure and frequencies

The first step is to find the ground state structure and calculate its frequencies to find the harmonic Helmholtz free energy. While it is impossible to prove that this is the lowest energy structure, the distribution of the 4000 optimized structures does provide some insights. If there are many bins (the bin size is set to 0.2 kJ/mol pfu) present in the plot, many nonequivalent local minima are present in the sampled phase space during the 150 K MD simulations. The more nonequivalent local minima, the less likely that the global minima can be found. The number of times the lowest observed minimum is found, indicates how likely it is to find it. If it is frequently found, then we could have performed fewer optimizations. If not, then the number of optimizations is definitely justified and more optimizations can be considered to affirm that this is the lowest energy structure.

Fig. S7 shows the histogram of the energies of all 4000 optimized structures for the $\gamma$ phase of $FAPbI_3$, with a simulation cell set to the average cell at 150 K. There are a lot of different optimized energies, indicating that there are a lot of nonequivalent local minima. The lowest energy was found a few times, which indicates that 4000 optimizations is definitely justified and might be enough. Moreover, the TI approach is in principle correct for a harmonic PES around random local minima. With the downside that the TI corrections might be more difficult to converge. See also Sec. 7, which discusses the histograms for all materials, phases, and simulation cells.

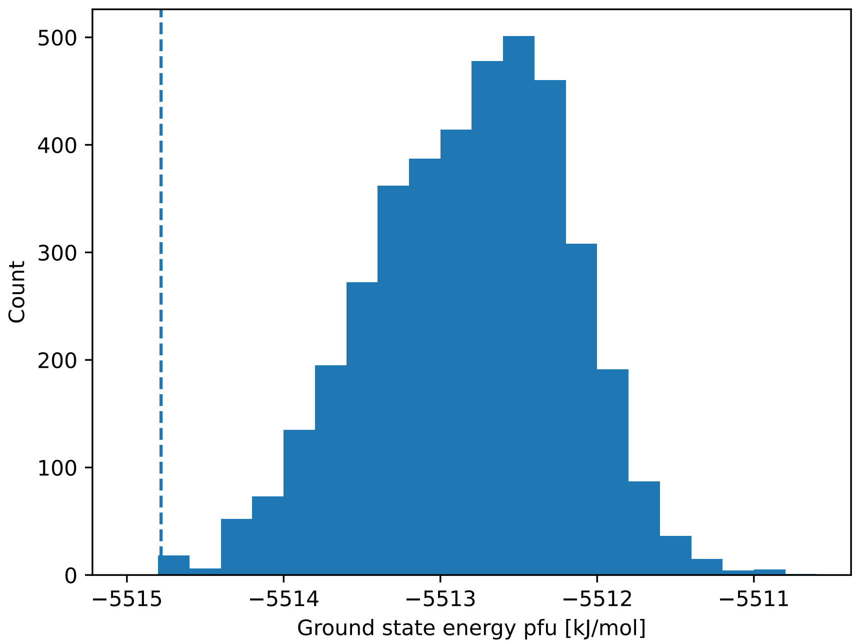


Figure S7: Histogram of the energies of all 4000 optimized structures for the $\gamma$ phase of $FAPbI_3$, with a simulation cell set to the average cell at 150 K. The dotted line indicates the lowest optimized energy.

We construct a harmonic PES around the lowest energy minima and calculate the harmonic free energy via its frequencies. Therefore, the Hessian matrix of the lowest energy structure is determined via finite displacements of 53 fm. If the mass-weighted Hessian has negative eigenvalues (besides the 3 translation modes that have eigenvalues close to zero), then a short MD simulation of 500 steps at 100 K are performed, using the lowest energy structure as the initial structure. The last structure of this MD simulation is then reoptimized and its mass-weighted Hessian is determined. If this matrix still has significant negative eigenvalues, the same MD simulation is performed starting from the last structure of the previous MD simulation. This procedure is followed until the mass-weighted Hessian no longer contains significant negative eigenvalues. These eigenvalues are the frequencies from which the harmonic free energy can be determined. The phonon spectra of the $\gamma$ phase of $FAPbI_3$, with a simulation cell set to the average cell at 150 K is visualized in Fig. S8.

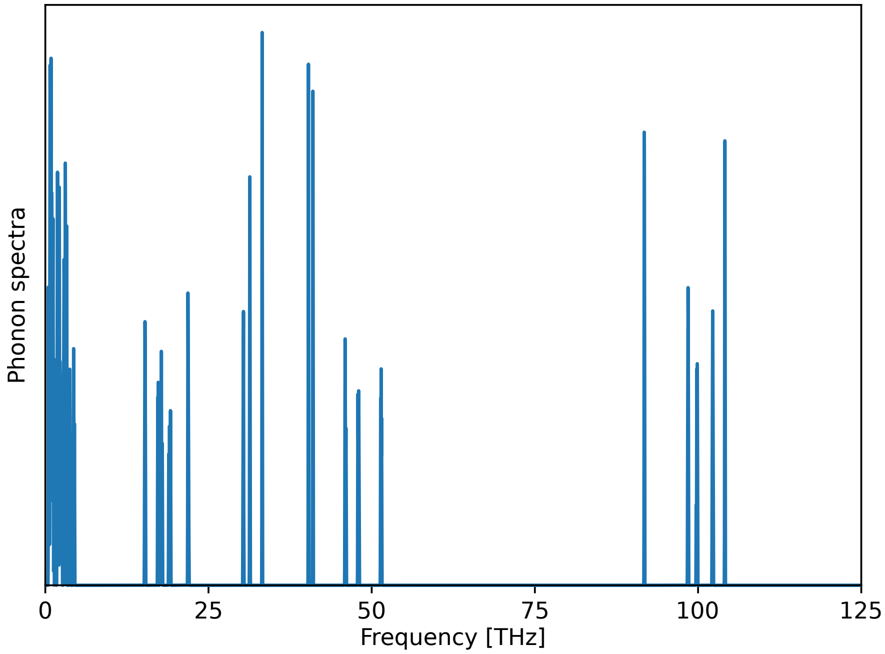


Figure S8: Phonon spectra for the $\gamma$ phase of $FAPbI_3$, with a simulation cell set to the average cell at 150 K. Gaussian smearing of 0.02 THz is added to the eigenvalues of the mass-weighted Hessian of the lowest energy structure to construct this spectrum.

### 5.2 Going from the harmonic to the intermediate PES

To calculate the free energy difference between two PES, a $\lambda$-TI contribution is determined. This contribution is calculated via the ensemble average of the energy difference between the two PES, which has to be determined for multiple ensembles that lie along a $\lambda$-path that gradually changes one PES into the other, *i.e.*, ensembles average for $U(\lambda) = U_{\text{begin}} + \lambda \left(U_{\text{end}} - U_{\text{begin}}\right)$. To investigate how the ensemble average changes along the $\lambda$-path, we plot the ensemble average and the standard error of the energy difference between the intermediate and harmonic PES as a function of $\lambda$ for the $\gamma$ phase of $FAPbI_3$, with a simulation cell set to the average cell at 150 K. The curve is smooth, monotonically decreasing, and the error bars are too small to be visible. These are signs that the free energy contribution has converged.

The curve shows non-linear behavior at the edges. Therefore, we took more $\lambda$ points near $\lambda = 0$ and $\lambda = 1$, see Sec. 3.3 of the manuscript. This plot also indicates that along the $\lambda$-path different phase spaces are sampled justifying the use of thermodynamic integration over free energy perturbation.[4]

When sampling in the harmonic PES, the intermediate PES is higher in energy, indicating

that the harmonic PES samples unlikely phase spaces of the MLP PES. A possible explanation could be that the translation modes of the FA molecule are relatively free to move leading to short distances between the organic atoms and the iodine atoms. The harmonic PES definitely sampled unrealistic structures, because the initial MLP trained on *ab initio* MD structures generated at 800 K failed to accurately predict some Hessian MD structures generated at 150 K. Therefore, extra Hessian structures got added to the *ab initio* data set, see Sec. 3.2.

On the contrary, when sampling the intermediate PES, the harmonic PES is higher in energy. This is probably the results of nearby local minima that are (partially) sampled for which the harmonic PES predicts a high energy. As shown in Sec. 5.4, for the MLP PES this effect is even more pronounced, because a lot more minima become accessible leading to a significantly negative free energy contribution.

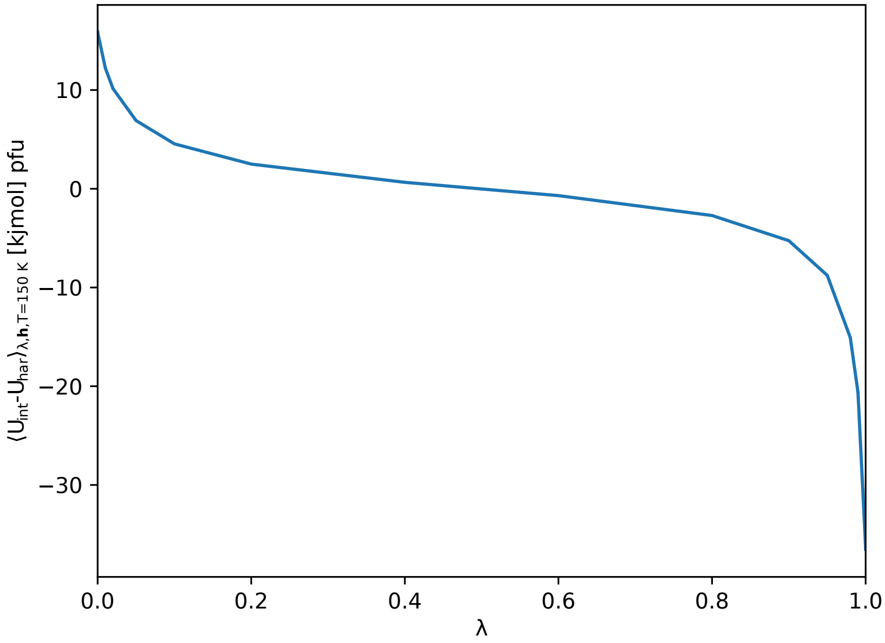


Figure S9: Ensemble average at 150 K of the energy difference between the intermediate PES and harmonic PES as a function of the interpolation parameter $\lambda$ for the $\gamma$ phase of $FAPbI_3$, with a simulation cell set to the average cell at 150 K.

## 5.3 Temperature correction to the Helmholtz free energy for the intermediate PES

For the temperature correction to the Helmholtz free energy we need to calculate the ensemble average of the energy at different temperatures. If we plot this ensemble average as a function of temperature we would observe an approximately linear relationship, similar to the ensemble

average of the harmonic PES, namely $\langle U \rangle_{\text{harm},T} = E_{\text{GS}} + (3N-3)\,\frac{k_{\text{B}}T}{2}$. Therefore, we investigate the anharmonic ensemble average of the energy:[5]

$$\langle U_{\text{anharm}} \rangle_{\text{int},T} = \langle U \rangle_{\text{int},T} - \langle U \rangle_{\text{harm},T}. \tag{S5.1}$$

As shown by Cheng and Ceriotti,[5] the Helmholtz free energy can then be determined as follows:

$$\frac{F_{\text{int}}(T_1)}{k_{\text{B}}T_1} = \frac{E_{\text{GS}}}{k_{\text{B}}T_1} + \frac{F_{\text{int}}(T_0) - E_{\text{GS}}}{k_{\text{B}}T_0} - (3N-3)\ln\frac{T_1}{T_0} - \int_{T_0}^{T_1} \frac{\langle U_{\text{anharm}} \rangle_{\text{int},T}}{k_{\text{B}}T^2} dT \tag{S5.2}$$

Because the third term is the same for each phase, the free energy differences between the phases will have a linear relationship with temperature if $\langle U_{\text{anharm}} \rangle_{\text{int},T} = 0$. This is also the case for the harmonic approximation, with the difference that $F_{\text{int}}(T_0)$ can already include anharmonic corrections calculated in Sec. 5.2. A $\lambda$-TI correction calculated at 150 K will be four times more important at 600 K.

The $\langle U_{\text{anharm}} \rangle_{\text{int},T}$ can be interpreted as an added correction on top of the $\lambda$-TI correction. This value impacts the slope of the Helmholtz free energy differences as a function of temperature, which is at $T_0$ equal to $\frac{\Delta F_{\text{int}}(T_0) - \Delta E_{\text{GS}}}{k_{\text{B}}T_0}$. Therefore, when $\langle U_{\text{anharm}} \rangle_T$ is much larger for one phase compared to another, then the free energy difference will have a significant curvature at temperature $T$.

The results for the $\gamma$ phase of $FAPbI_3$, with a simulation cell set to the average cell at 150 K is shown in Fig. S10. The ensemble average of the anharmonic energy for the intermediate PES is small. This means that the anharmonicity of the intermediate PES (if present) was already captured at 150 K via $\lambda$-TI, see Sec. 5.2.

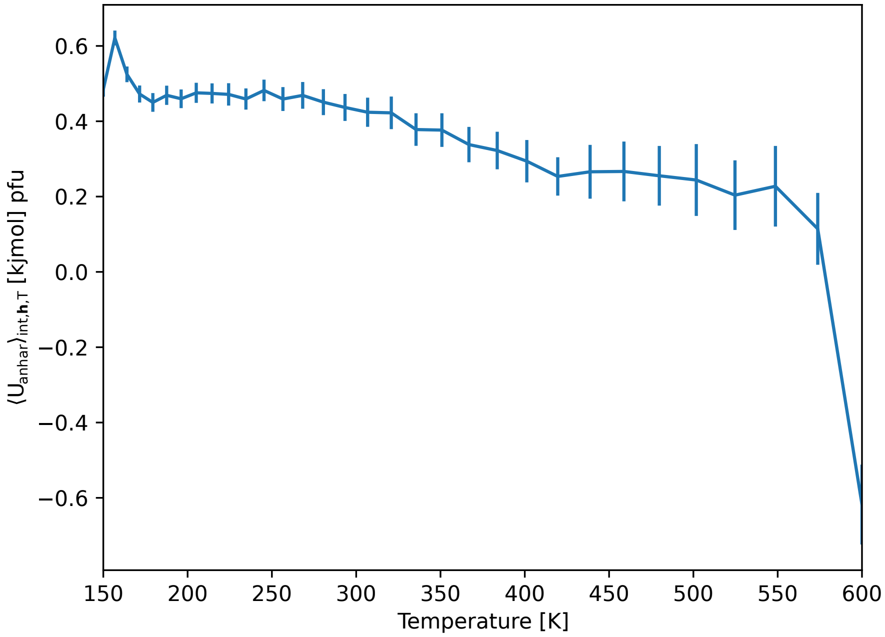


Figure S10: Ensemble average of the anharmonic energy of the intermediate PES as a function of the temperature for the $\gamma$ phase of $FAPbI_3$, with a simulation cell set to the average cell at 150 K.

### 5.4 Going from the intermediate to the MLP PES

For the organic molecules the intermediate PES is the MLP with a positive bias, so the ensemble average of the energy difference is always negative. When $\lambda$ approaches 1, the bias loses its effect and the other minima become accessible leading to a larger energy difference between the intermediate and MLP PES. Fig. S11 plots the ensemble average of the energy difference between the MLP and intermediate PES as a function of $\lambda$. Due to multiple local minima, the correction is rather large. Therefore, it is important to include enough $\lambda$ values near $\lambda = 1$, and to perform multiple long MD simulations. The small error bars indicate that the ensemble averages are converged.

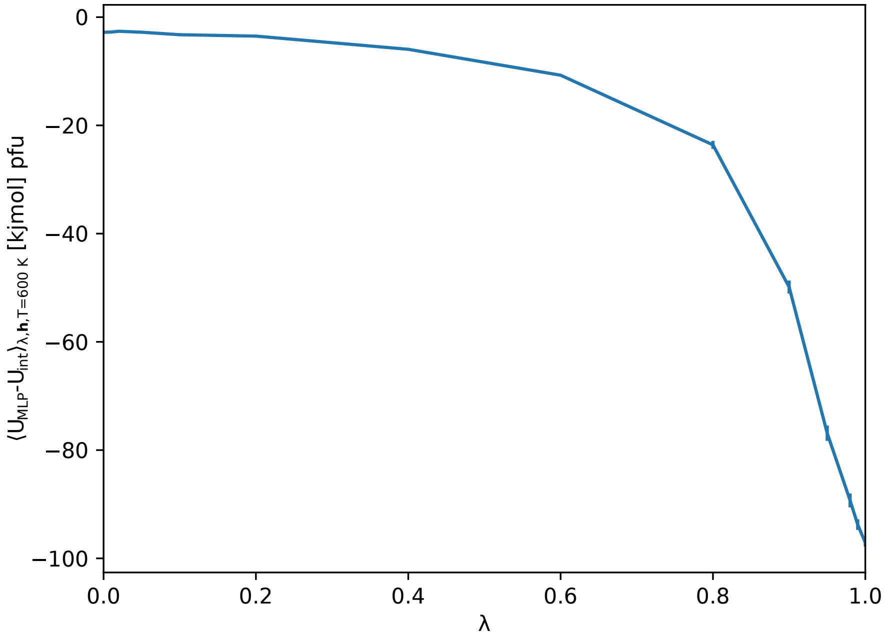


Figure S11: Ensemble average at 600 K of the energy difference between the MLP PES and intermediate PES as a function of the interpolation parameter $\lambda$ for the $\gamma$ phase of $FAPbI_3$ with a simulation cell set to the average cell at 150 K.

## 5.5 Temperature correction to the Helmholtz free energy for the MLP PES

The same analysis as in Sec. 5.3 is performed for the MLP PES, the results are plotted in Fig. S12. The anharmonic energy is higher than for the intermediate PES. If a local minimum is already well sampled at low temperatures then its effect on the free energy is already captured via the second term of Eq. S5.2 by the determination of $F_{\text{int}}\left(T_{\text{low}}\right)$. If a local minimum becomes relevant at a specific temperature, then the free energy is lower than the free energy of a system without this local minimum. This lowering effect on the free energy can be achieved via an increase of $\langle U_{\text{anharm}} \rangle_{\text{MLP}}$. We cannot directly link the magnitude of $\langle U_{\text{anharm}} \rangle_{\text{MLP},T}$ to the number of local minima that are getting sampled around this temperature, because the anharmonicity of the already sampled minima also has influence.

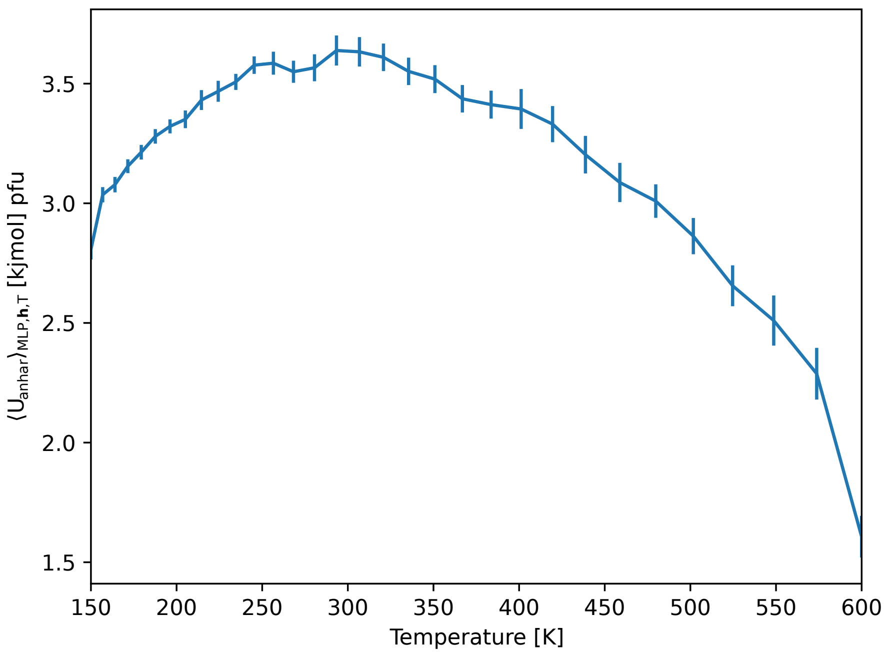


Figure S12: Ensemble average of the anharmonic energy of the MLP PES as a function of the temperature for the $\gamma$ phase of $FAPbI_3$, with a simulation cell set to the average cell at 150 K.

## 5.6 Going from Helmholtz to Gibbs free energy

To go from the Helmholtz free energy at a specific simulation cell to the Gibbs free energy at a specific pressure we need to determine the probability of this simulation cell at this pressure, see also Eq. 2.6 in the manuscript. Because the probability of the six-dimensional simulation cell is difficult to determine, we use the probability of the volume instead. The probability of encountering the volume at a specific temperature and pressure is determined via NPT MD simulations at those conditions and by creating a histogram of the volumes with a bin size of 0.1 Å$^3$ pfu. Fig. S13 shows the results for a NPT MD simulation at 150 K and 0.1 MPa for the $\gamma$ phase of $FAPbI_3$. The probability is determined by the normalized magnitude of the bin that contains the volume of the used simulation cell. Because the histogram contains a bit of noise, we calculate the running average with a window of 9 and use the value at the volume of the simulation cell. This probability is close to the maximum probability because we used the average simulation cell of the NPT MD simulations to determine the Helmholtz free energy.

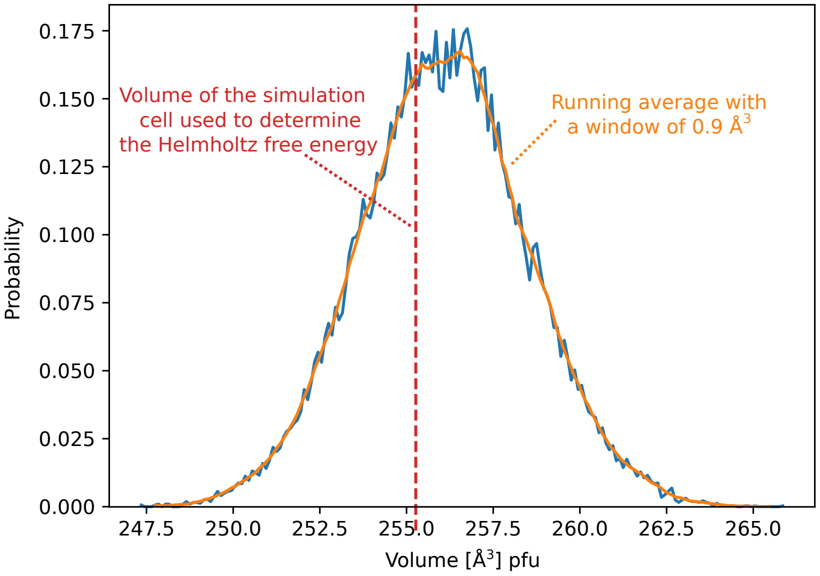


Figure S13: Probability distribution of the volume during a NPT MD simulation at 150 K and 0.1 MPa for the $\gamma$ phase of $FAPbI_3$. The probability is estimated via a histogram with 0.1 Å$^3$ as the bin size shown in blue. To decrease the noise on the histogram a running average with a window of 9 is shown in orange. The volume of the simulation cell used to determine the Helmholtz free energy is indicated by the vertical red dotted line.

## 5.7 Temperature correction to the Gibbs free energy for the MLP PES

The same analysis as in Sec. 5.5 is performed, except instead of the energy the anharmonic enthalpy is investigated. The anharmonic enthalpy is defined as follows:

$$\langle H_{\text{anharm}} \rangle_{\text{int},T} = \langle H \rangle_{\text{int},T} - \langle H \rangle_{\text{harm},T}, \tag{S5.3}$$

where $H = U + PV$, is the enthalpy of a structure, and $\langle H \rangle_{\text{harm},T} = H_{\text{GS}} + (3N-3)\frac{k_B T}{2}$. Fig. S14 plots the ensemble average of the anharmonic enthalpy of the MLP PES for the $\gamma$ phase of $FAPbI_3$ at atmospheric pressure. The ensemble average is higher for the enthalpy in NPT simulations than for the energy in the NVT simulations. An observation that is valid for all phases and all materials investigated in this work. This can be caused by the extra cell degrees of freedom not included in the definition of the harmonic enthalpy.

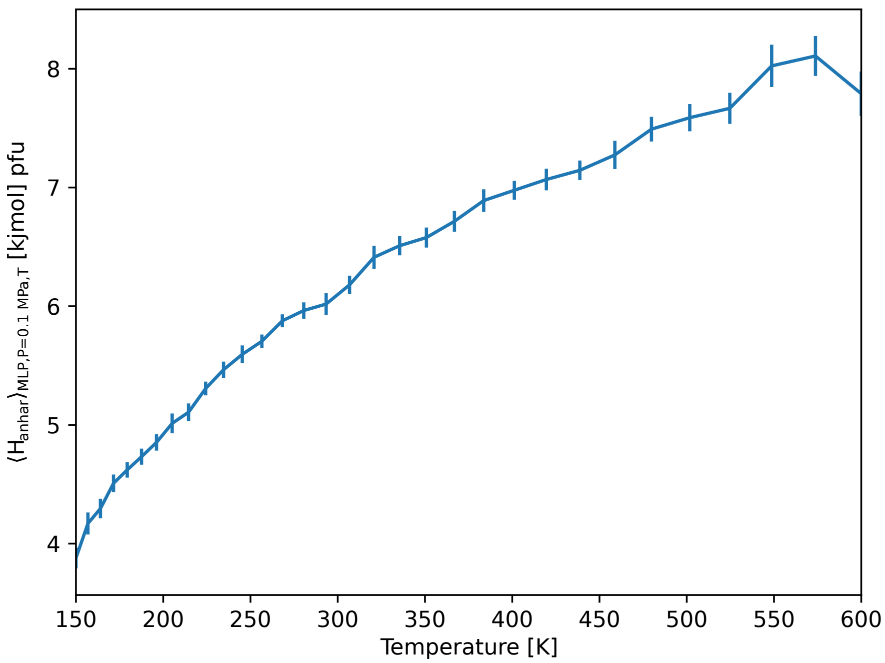


Figure S14: Ensemble average of the anharmonic enthalpy of the MLP PES as a function of the temperature for the $\gamma$ phase of $FAPbI_3$ at atmospheric pressure.

## 5.8 Spectra from NVE MD simulations

As an alternative to the TI approach, the Helmholtz free energy can be determined using NVE MD simulations.[3] Figure S15 presents the phonon spectrum for the $\gamma$ phase of $FAPbI_3$, with the simulation cell set to the average structure at 150 K. Compared to the spectrum obtained via the Hessian matrix (see Fig. S8), we observe that the peaks are broadened.

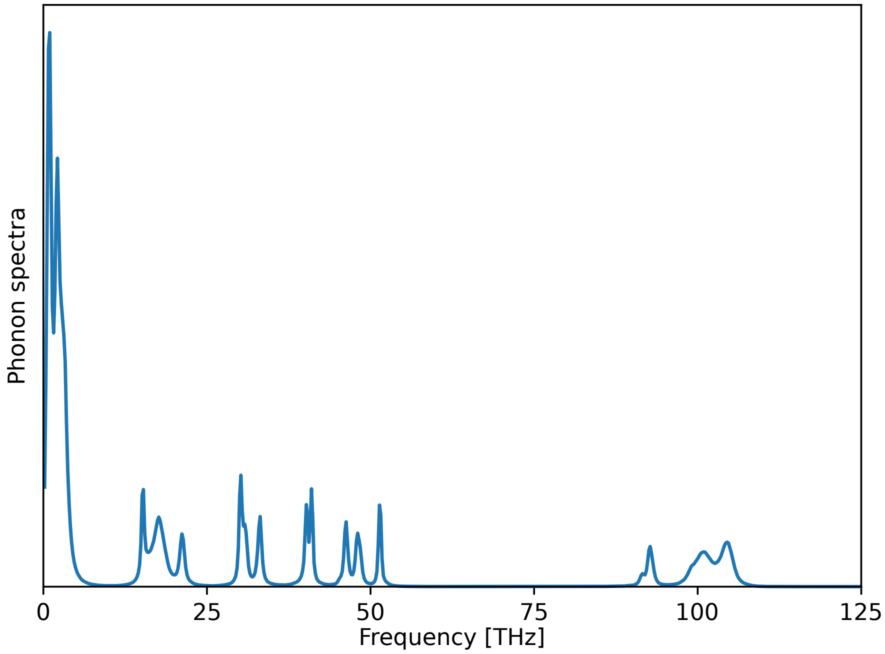


Figure S15: Phonon spectra for the $\gamma$ phase of $FAPbI_3$, with a simulation cell set to the average cell at 150 K. This spectrum is calculated from NVE MD simulations at 150 K.

# 6 Parameters of the average cell used to calculate the Helmholtz free energy

Tabs. S4 ($CsPbI_3$), S5 ($FAPbI_3$), and S6 ($MAPbI_3$) present the parameters of the average simulation cell, containing 8 formula units, used to calculate the Helmholtz free energy. These parameters were obtained from NPT MD simulations at the specified temperature and a pressure of 0.1 MPa. Fig. S16 plots the volumes as a function of temperature. The volume is larger when the A-site cation is larger. For each material, the volumes of the phases are similar, only for the $\delta_{Cs}$ phase of $CsPbI_3$ is the volume significantly lower. As discussed in Sec. 4.3 of the manuscript, at low temperatures the orientational freedom of the MA molecules is more restricted than at higher temperatures. A possible explanation could be the volume of the simulation cell at 150 K, which is significantly lower than at the higher temperatures. This also explains why the FA molecules at lower temperatures are more free to rotate than the MA molecules, because the volume of the simulation cell of $FAPbI_3$ at 150 K is significantly larger, see Sec. 9.

Since the simulation cells containing 64 formula units are constructed as $2 \times 2 \times 2$ supercells of those with 8 formula units, their parameters are not presented here.

Table S4: Cell parameters for the NVT simulation of $CsPbI_3$ containing 8 formula units.

| Phase | Average cell at temperature | $\lvert\vec{a}\rvert$ [Å] | $\lvert\vec{b}\rvert$ [Å] | $\lvert\vec{c}\rvert$ [Å] | $\alpha$ [°] | $\beta$ [°] | $\gamma$ [°] | Volume pfu [Å$^3$] |
|---|---|---|---|---|---|---|---|---|
| $\gamma$ | 0 | 12.32 | 12.32 | 12.5 | 90.0 | 90.0 | 86.7 | 237.0 |
| | 150 | 12.56 | 12.4 | 12.4 | 87.84 | 89.98 | 90.01 | 241.0 |
| | 187 | 12.61 | 12.41 | 12.4 | 88.01 | 90.06 | 90.02 | 242.0 |
| | 234 | 12.45 | 12.62 | 12.43 | 89.95 | 91.28 | 89.99 | 244.0 |
| | 293 | 12.62 | 12.46 | 12.51 | 90.56 | 89.99 | 89.73 | 246.0 |
| | 350 | 12.65 | 12.52 | 12.53 | 90.26 | 90.14 | 90.05 | 248.0 |
| | 419 | 12.6 | 12.57 | 12.64 | 89.89 | 90.1 | 90.13 | 250.0 |
| | 501 | 12.61 | 12.65 | 12.68 | 90.11 | 89.98 | 90.02 | 253.0 |
| | 600 | 12.68 | 12.67 | 12.73 | 90.01 | 90.03 | 90.03 | 256.0 |
| $\delta_{Cs}$ | 0 | 17.8 | 10.39 | 9.59 | 90.0 | 90.0 | 90.0 | 221.0 |
| | 150 | 17.91 | 10.47 | 9.63 | 89.98 | 90.05 | 89.99 | 226.0 |
| | 187 | 17.94 | 10.5 | 9.64 | 90.02 | 90.02 | 89.99 | 227.0 |
| | 234 | 17.98 | 10.52 | 9.65 | 89.98 | 90.04 | 89.98 | 228.0 |
| | 293 | 18.03 | 10.56 | 9.67 | 90.0 | 90.04 | 89.97 | 230.0 |
| | 350 | 18.08 | 10.59 | 9.7 | 89.98 | 90.03 | 89.9 | 232.0 |
| | 419 | 18.15 | 10.63 | 9.72 | 89.98 | 90.04 | 89.96 | 234.0 |
| | 501 | 18.24 | 10.68 | 9.76 | 89.96 | 89.99 | 89.92 | 237.0 |
| | 600 | 18.36 | 10.73 | 9.81 | 89.96 | 90.05 | 89.96 | 241.0 |
| $\delta_{FA}$ | 0 | 16.01 | 13.91 | 8.43 | 90.0 | 90.0 | 90.0 | 235.0 |
| | 150 | 15.89 | 14.23 | 8.48 | 89.96 | 89.88 | 89.97 | 240.0 |
| | 187 | 15.85 | 14.34 | 8.49 | 89.98 | 90.01 | 89.96 | 241.0 |
| | 234 | 15.83 | 14.43 | 8.5 | 90.01 | 89.58 | 90.13 | 243.0 |
| | 293 | 15.81 | 14.57 | 8.51 | 90.06 | 89.65 | 90.86 | 245.0 |
| | 350 | 15.75 | 14.76 | 8.51 | 90.03 | 89.66 | 90.84 | 247.0 |
| | 419 | 15.78 | 14.86 | 8.53 | 89.94 | 89.03 | 91.51 | 250.0 |
| | 501 | 15.82 | 14.96 | 8.56 | 89.88 | 89.14 | 90.7 | 253.0 |
| | 600 | 15.91 | 15.07 | 8.6 | 89.68 | 89.75 | 90.51 | 258.0 |

Table S5: Cell parameters for the NVT simulation of $FAPbI_3$ containing 8 formula units.

| Phase | Average cell at temperature | $\|\vec{a}\|$ [Å] | $\|\vec{b}\|$ [Å] | $\|\vec{c}\|$ [Å] | $\alpha$ [°] | $\beta$ [°] | $\gamma$ [°] | Volume pfu [Å$^3$] |
|---|---|---|---|---|---|---|---|---|
| $\gamma$ | 0 | 12.59 | 12.76 | 12.59 | 90.0 | 92.8 | 90.0 | 253.0 |
| | 150 | 12.62 | 12.67 | 12.77 | 90.09 | 90.32 | 90.16 | 255.0 |
| | 187 | 12.73 | 12.72 | 12.77 | 89.43 | 89.7 | 89.62 | 258.0 |
| | 234 | 12.8 | 12.72 | 12.7 | 90.17 | 90.27 | 89.94 | 258.0 |
| | 293 | 12.78 | 12.81 | 12.79 | 90.24 | 90.41 | 89.96 | 262.0 |
| | 350 | 12.81 | 12.86 | 12.81 | 89.99 | 90.09 | 89.77 | 264.0 |
| | 419 | 12.85 | 12.89 | 12.85 | 89.83 | 89.66 | 89.73 | 266.0 |
| | 501 | 12.9 | 12.92 | 12.87 | 89.74 | 89.94 | 89.92 | 268.0 |
| | 600 | 12.95 | 12.98 | 12.94 | 89.96 | 89.95 | 89.8 | 272.0 |
| $\delta_{Cs}$ | 0 | 19.05 | 11.7 | 9.08 | 90.0 | 87.84 | 90.0 | 253.0 |
| | 150 | 19.49 | 11.55 | 9.21 | 91.14 | 89.2 | 90.0 | 259.0 |
| | 187 | 19.5 | 11.71 | 9.14 | 89.23 | 90.55 | 89.75 | 261.0 |
| | 234 | 19.55 | 11.74 | 9.16 | 88.92 | 89.63 | 91.61 | 263.0 |
| | 293 | 19.7 | 11.73 | 9.17 | 89.99 | 90.36 | 91.09 | 265.0 |
| | 350 | 19.77 | 11.67 | 9.24 | 90.68 | 89.81 | 89.55 | 267.0 |
| | 419 | 19.77 | 11.74 | 9.27 | 88.77 | 90.23 | 89.64 | 269.0 |
| | 501 | 19.88 | 11.74 | 9.35 | 89.51 | 90.12 | 89.94 | 273.0 |
| | 600 | 19.91 | 11.85 | 9.36 | 90.07 | 90.22 | 89.44 | 276.0 |
| $\delta_{FA}$ | 0 | 15.69 | 15.1 | 8.46 | 90.0 | 90.0 | 90.0 | 251.0 |
| | 150 | 15.75 | 15.34 | 8.59 | 89.48 | 90.41 | 92.5 | 259.0 |
| | 187 | 15.88 | 15.11 | 8.62 | 89.85 | 89.54 | 90.27 | 258.0 |
| | 234 | 15.82 | 15.17 | 8.73 | 90.1 | 91.72 | 88.67 | 262.0 |
| | 293 | 15.88 | 15.2 | 8.73 | 90.03 | 91.55 | 90.77 | 263.0 |
| | 350 | 15.95 | 15.31 | 8.71 | 89.96 | 90.96 | 90.83 | 266.0 |
| | 419 | 15.93 | 15.45 | 8.77 | 89.69 | 91.24 | 91.46 | 270.0 |
| | 501 | 16.01 | 15.46 | 8.83 | 89.82 | 90.76 | 90.13 | 273.0 |
| | 600 | 16.06 | 15.66 | 8.91 | 89.9 | 89.64 | 90.5 | 280.0 |

Table S6: Cell parameters for the NVT simulation of $MAPbI_3$ containing 8 formula units.

| Phase | Average cell at temperature | $\|\vec{a}\|$ [Å] | $\|\vec{b}\|$ [Å] | $\|\vec{c}\|$ [Å] | $\alpha$ [°] | $\beta$ [°] | $\gamma$ [°] | Volume pfu [$Å^3$] |
|---|---|---|---|---|---|---|---|---|
| $\gamma$ | 0 | 12.29 | 12.29 | 12.69 | 90.0 | 90.0 | 87.46 | 240.0 |
| | 150 | 12.27 | 12.43 | 12.74 | 90.05 | 90.04 | 90.1 | 243.0 |
| | 187 | 12.62 | 12.52 | 12.65 | 90.17 | 89.47 | 89.99 | 250.0 |
| | 234 | 12.69 | 12.59 | 12.59 | 89.89 | 90.72 | 90.24 | 251.0 |
| | 293 | 12.64 | 12.62 | 12.7 | 90.4 | 90.33 | 89.41 | 253.0 |
| | 350 | 12.67 | 12.69 | 12.67 | 90.47 | 90.21 | 90.05 | 255.0 |
| | 419 | 12.67 | 12.67 | 12.83 | 89.93 | 89.3 | 89.84 | 257.0 |
| | 501 | 12.74 | 12.73 | 12.82 | 90.27 | 90.12 | 89.78 | 260.0 |
| | 600 | 12.81 | 12.81 | 12.83 | 90.06 | 89.95 | 89.72 | 263.0 |
| $\delta_{Cs}$ | 0 | 18.54 | 11.02 | 9.52 | 90.0 | 90.0 | 90.0 | 243.0 |
| | 150 | 19.18 | 10.82 | 9.4 | 89.88 | 90.31 | 90.2 | 244.0 |
| | 187 | 19.2 | 10.89 | 9.38 | 90.04 | 90.42 | 90.0 | 245.0 |
| | 234 | 18.64 | 11.31 | 9.39 | 90.03 | 90.28 | 90.52 | 247.0 |
| | 293 | 19.33 | 10.87 | 9.44 | 90.26 | 90.13 | 89.35 | 248.0 |
| | 350 | 19.22 | 10.95 | 9.52 | 90.26 | 90.14 | 90.11 | 250.0 |
| | 419 | 19.12 | 11.06 | 9.57 | 90.52 | 89.87 | 91.05 | 253.0 |
| | 501 | 19.17 | 11.12 | 9.63 | 90.18 | 89.89 | 89.11 | 257.0 |
| | 600 | 19.22 | 11.17 | 9.73 | 90.1 | 89.71 | 90.54 | 261.0 |
| $\delta_{FA}$ | 0 | 15.75 | 14.67 | 8.49 | 86.07 | 90.0 | 90.0 | 245.0 |
| | 150 | 15.72 | 14.91 | 8.49 | 88.52 | 94.44 | 89.65 | 248.0 |
| | 187 | 15.73 | 14.89 | 8.51 | 89.18 | 93.25 | 89.62 | 249.0 |
| | 234 | 15.75 | 14.9 | 8.54 | 89.53 | 88.41 | 90.12 | 250.0 |
| | 293 | 15.72 | 14.97 | 8.6 | 90.05 | 88.42 | 89.4 | 253.0 |
| | 350 | 15.73 | 14.98 | 8.66 | 89.7 | 90.21 | 88.47 | 255.0 |
| | 419 | 15.81 | 15.04 | 8.67 | 89.83 | 90.49 | 89.5 | 258.0 |
| | 501 | 15.85 | 15.16 | 8.68 | 89.82 | 89.62 | 89.47 | 261.0 |
| | 600 | 15.93 | 15.23 | 8.75 | 89.86 | 90.33 | 89.98 | 265.0 |

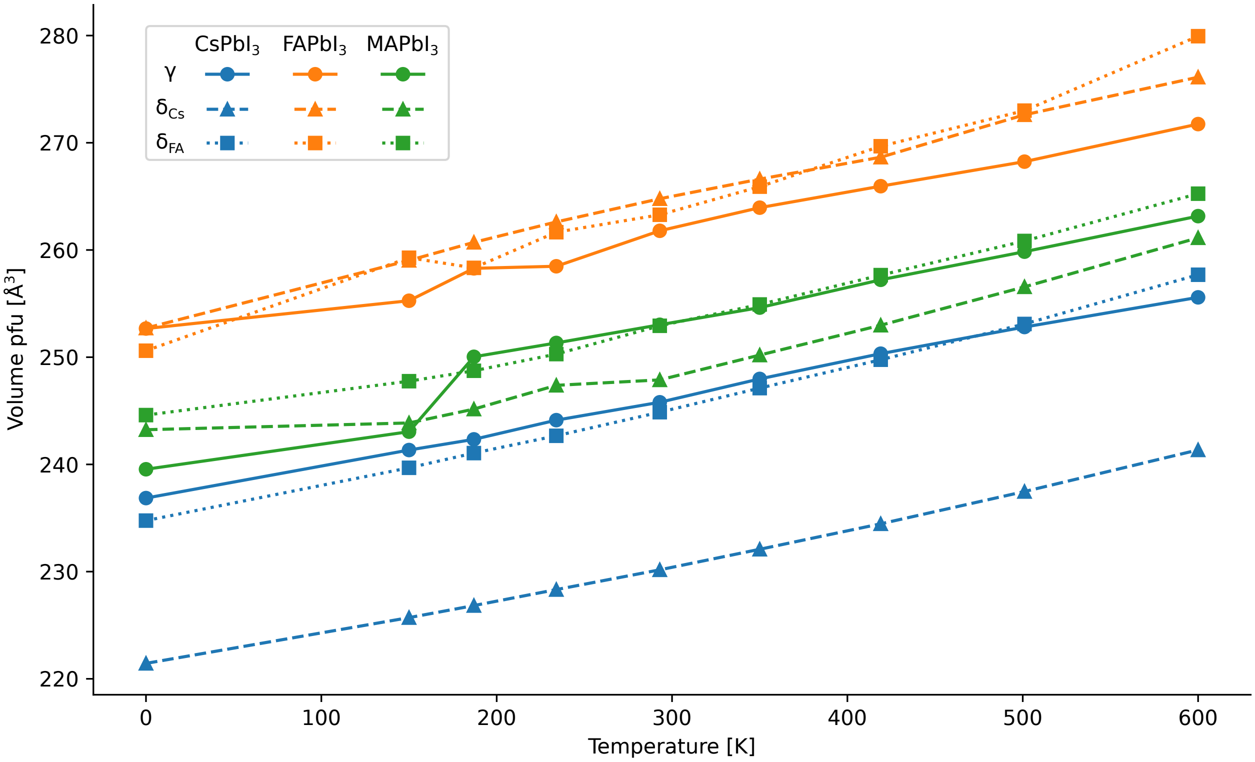


Figure S16: Volume of the average simulation cell in NPT at 0.1 MPa as a function of temperature for the three phases of $CsPbI_3$, $FAPbI_3$, and $MAPbI_3$.

# 7 Histogram of optimized energies

Figs. S17 ($CsPbI_3$), S18 ($FAPbI_3$), and S19 ($MAPbI_3$) present the histograms of the optimized energies keeping the simulation cell fixed at different temperatures. For each histogram, the optimizations were performed on 4000 initial structures that were generated via NVT (NPT) MD simulations at 150 K (and 0.1 MPa). To escape local minima, these MD simulations were coupled via REX with 31 simulations at higher temperatures, reaching a maximum of 600 K. For all phases and simulation cells of $CsPbI_3$, the 4000 optimizations resulted in approximately the same energy, while for $FAPbI_3$ and $MAPbI_3$ the energy distribution is broader. This is the result of the organic molecules which create multiple minima due to their orientation. For most simulations and phases of $MAPbI_3$ the lowest energy has (almost) the highest probability to be found, while for $FAPbI_3$ the lowest energy has a rather low probability. Only the lowest energy for the $\delta_{Cs}$ phase of $FAPbI_3$ has a good probability to be found.

In Sec. 9 the possible orientations of the organic molecules are plotted for the three phases of $FAPbI_3$ and $MAPbI_3$. At 150 K the possible orientations of the organic molecules are more restricted for $MAPbI_3$ than for $FAPbI_3$, and of the three phases of $FAPbI_3$ the FA molecules have the least freedom in the $\delta_{Cs}$ phase. A smaller phase space for the organic molecules correlates with a higher probability of finding the lowest energy. Therefore, it was crucial to choose initial structures from MD simulation at 150 K that were coupled with higher-temperature MD simulation via REX to escape local minima.

There are two options to improve the probability of finding the lowest energy. Namely, performing REX MD simulations with a lower minimal temperature to eliminate higher energy local minima, and performing more optimization. However, given the maximum temperature of our REX simulations is 600 K, 150 K as a minimum temperature is at the limit to assure a proper acceptance rate for 32 replicas. Moreover, given that we perform optimizations for 3 materials, 3 phases, 8 simulation cells containing 8 formula units, and 3 simulation cells containing 3 formula units, 4000 optimizations are at the limit of our computational resources. In principle, the TI approach is valid for any harmonic PES around random local minima. Therefore, it is not necessary to use the global minima. However, the TI corrections might be more difficult to converge.

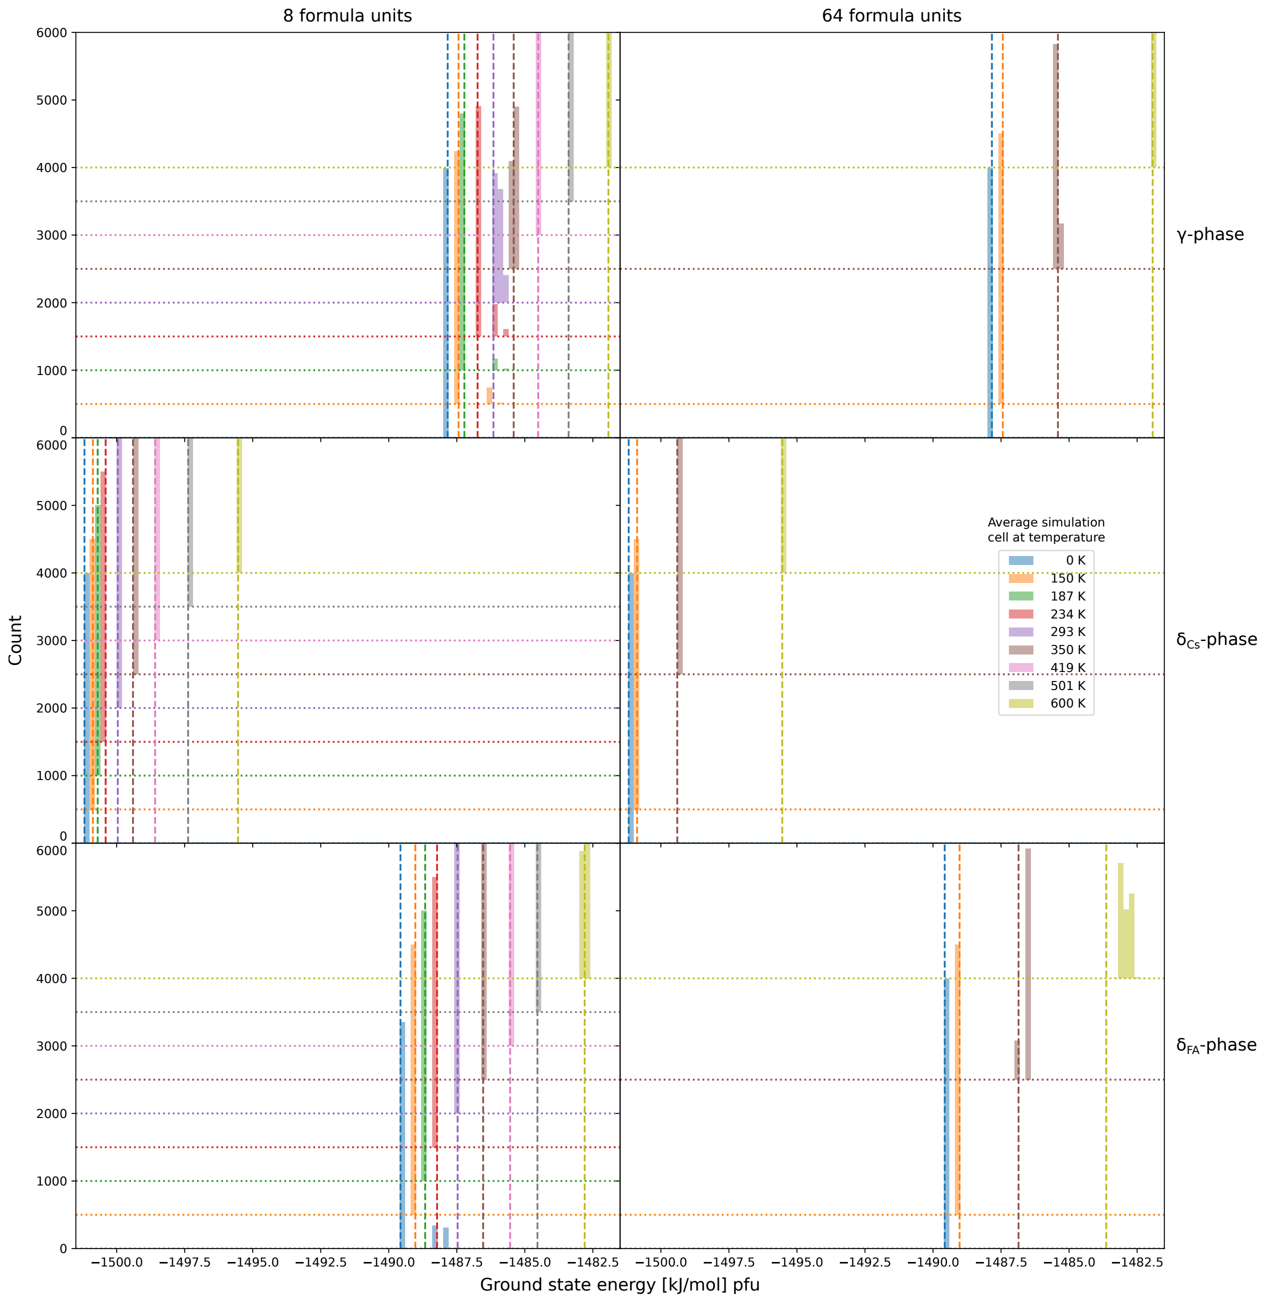


Figure S17: Histograms with a bin size of 0.2 kJ/mol pfu for the energy of 4000 optimized structures of $CsPbI_3$. The results for the three phases containing 8 and 64 formula units are shown. The blue histograms (*i.e.* 0 K) show the results for a full cell optimization, while the other optimizations kept the simulation cell fixed to the average cell at the specified temperature and at 0.1 MPa.

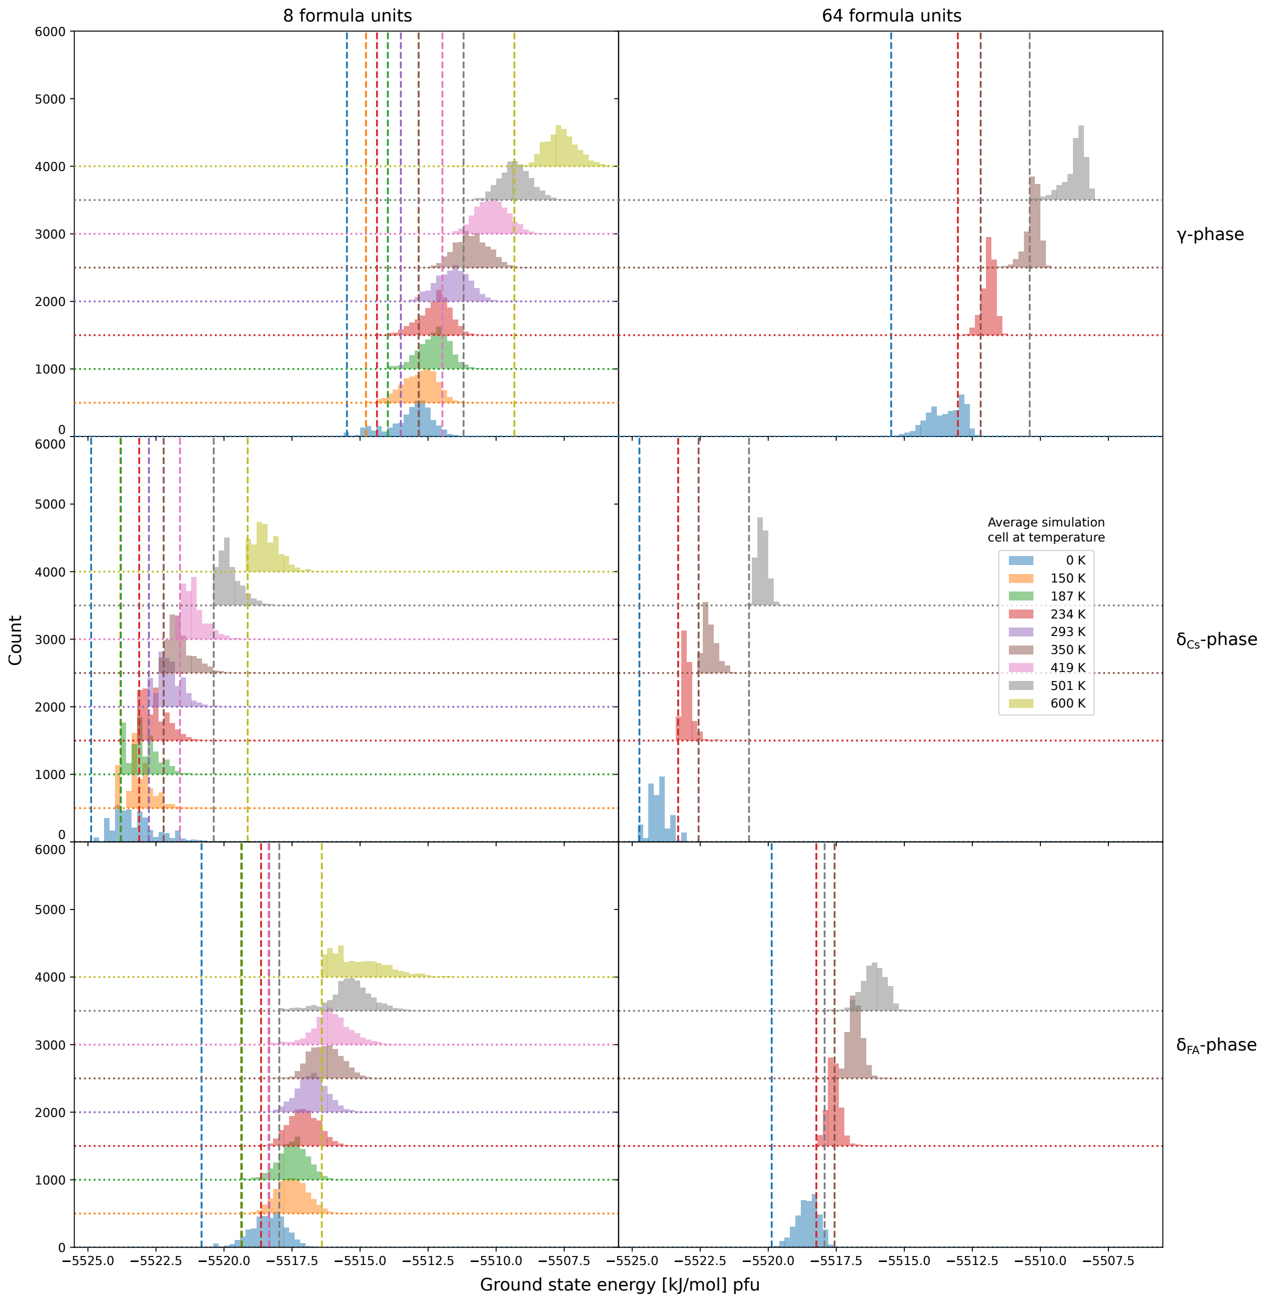


Figure S18: Histograms with a bin size of 0.2 kJ/mol pfu for the energy of 4000 optimized structures of $FAPbI_3$. The results for the three phases containing 8 and 64 formula units are shown. The blue histograms (*i.e.* 0 K) show the results for a full cell optimization, while the other optimizations kept the simulation cell fixed to the average cell at the specified temperature and at 0.1 MPa.

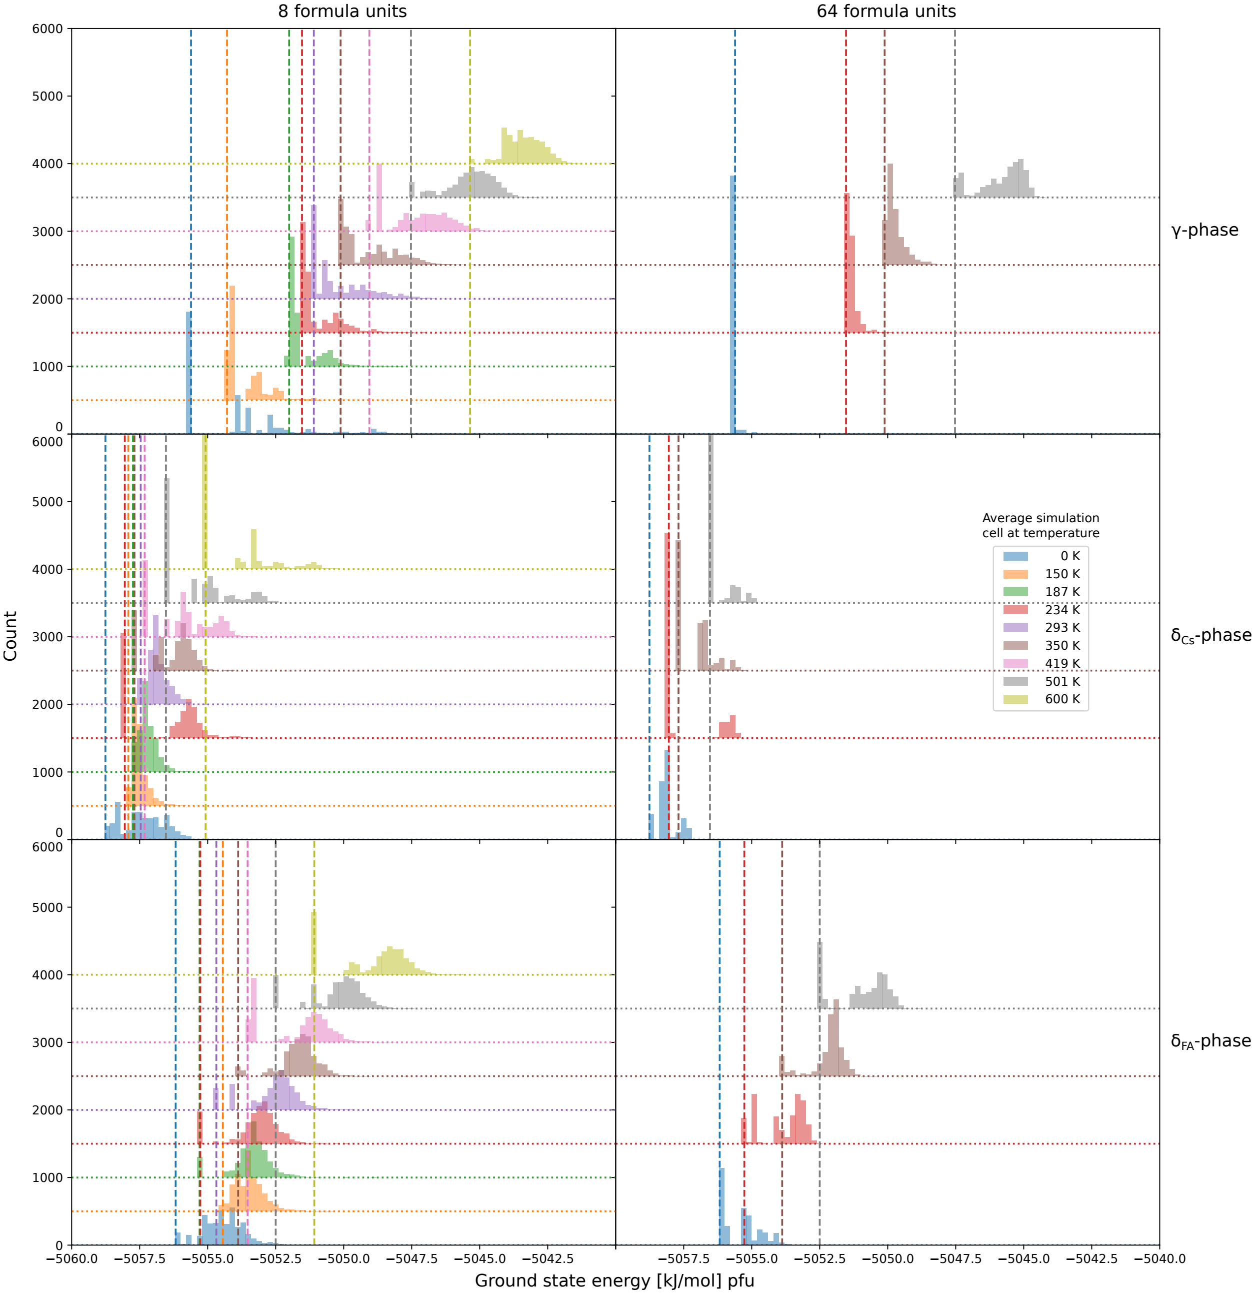


Figure S19: Histograms with a bin size of 0.2 kJ/mol pfu for the energy of 4000 optimized structures of $MAPbI_3$. The results for the three phases containing 8 and 64 formula units are shown. The blue histograms (*i.e.* 0 K) show the results for a full cell optimization, while the other optimizations kept the simulation cell fixed to the average cell at the specified temperature and at 0.1 MPa.

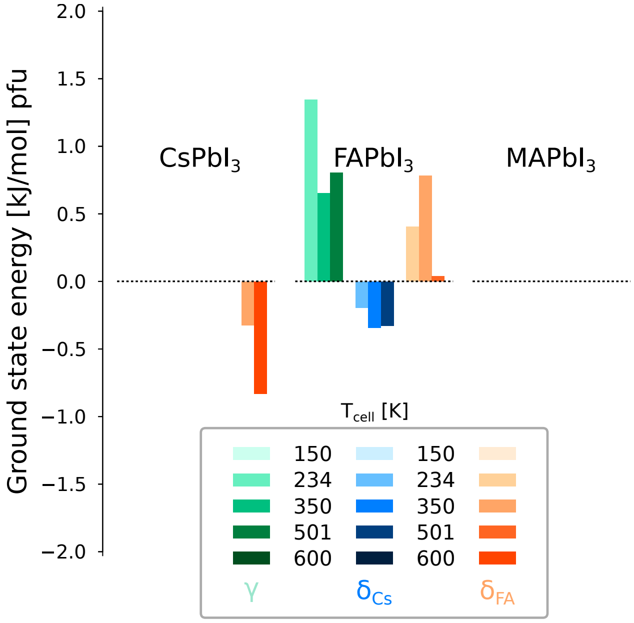


Figure S20: Ground state energy difference between optimized structures for 64 and 8 formula units.

Fig. S20 shows the differences between the lowest energy found for 64 and 8 formula units. Because the phase space is significantly larger for the 64 formula units, the probability of not finding the lowest energy is higher. Given the low probability of finding the lowest energy for the $\gamma$ and $\delta_{\mathrm{FA}}$ phases of $FAPbI_3$ containing 8 formula units, the optimization on 64 formula units failed to find this energy. Therefore, we opted to use the $2 \times 2 \times 2$ supercells of the lowest energy structure for 8 formula units to construct a harmonic PES for 64 formula units. Only the supercells for the $\delta_{\mathrm{FA}}$ phase of $CsPbI_3$ and the $\delta_{\mathrm{Cs}}$ phase of $FAPbI_3$ could optimize to a lower energy. For those systems, we did not use the lowest energy structure. However, this does not necessarily introduce errors because the TI approach can correct this.

## 8 Supercell effect on the free energy contributions

Fig. S21 shows the free energy difference between the $\delta$ phases and the $\gamma$ phase as a function of temperature in different PESs for simulation cells containing 64 formula units. The uncertainty due to the simulation cell is almost negligible for the Helmholtz and Gibbs free energies, only $CsPbI_3$ has a small dependence. We only performed the supercell simulation for three different simulation cells due to the high computational cost, which could hide larger discrepancies for different simulation cells. However, it appears that the cell degrees of freedom are not that relevant for a simulation cell containing 64 formula units. This is not surprising because there are only six cell degrees of freedom compared to 960 ($CsPbI_3$) or 2304 ($FAPbI_3$ and $MAPbI_3$) atomic degrees of freedom.

Compared to the results for eight formula units (see Fig. 6 in the manuscript), the Helmholtz and Gibbs free energy is higher for the $\gamma$ phase compared to the $\delta$ phases, which increases the transition temperatures. Fig. S22 shows the effect of the supercell on the six contributions to the Helmholtz free energy for each phase, and Fig. S23 shows the effect of the supercell on the energy difference with respect to the $\gamma$ phase. The ground state energy is not influenced because we used the $2 \times 2 \times 2$ supercells of the lowest energy structure for 8 formula units, see Sec. 7. The supercell leads to lower harmonic free energies for each phase, which can be explained by comparing the frequency spectra, see Fig. S24. The supercell has modes with lower frequencies that have a lower harmonic free energy, see Eq. 2.5 in the manuscript. This stabilizing effect is larger for the $\delta$ phases compared to the $\gamma$ phase. However, the anharmonic contribution partly counteracts this stability difference between the $\gamma$ and $\delta$ phases. Because the supercell positively affects the anharmonic corrections of the $\gamma$ phase and not the $\delta$ phases. The supercell has on average a destabilizing effect on the configurational free energy, because the number of minima do not scale exponentially with system size. This destabilizing effect is the largest for the $\gamma$ phase because the tilt of one octahedra influences the tilts of the other octahedra. Irregular tilting patterns lead to higher energies and thereby higher free energies.

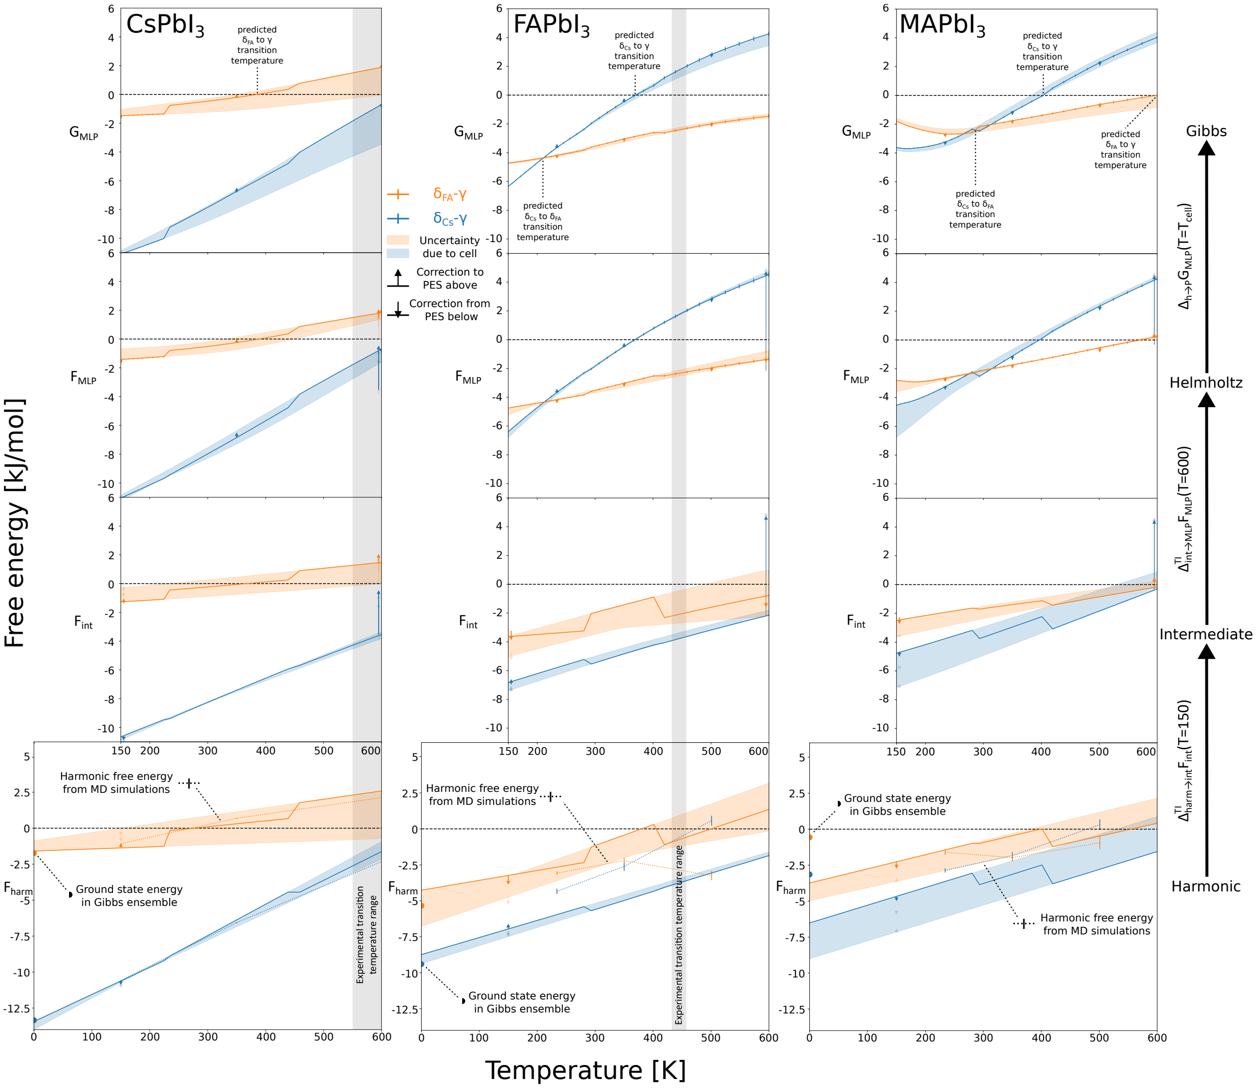


Figure S21: Free energy difference of the $\delta_{\mathrm{Cs}}$ (blue) and $\delta_{\mathrm{FA}}$ (orange) phases relative to the $\gamma$ phase as a function of temperature, computed using different PES: harmonic (via NVE MD simulations, dashed lines, and via Hessian calculations, solid lines with shaded areas), intermediate, and MLP. The Helmholtz and Gibbs free energies for the MLP PES are obtained from MD simulations in the NVT and NPT ensembles, respectively. The results correspond to simulation cells containing 64 formula units of $CsPbI_3$, $FAPbI_3$, and $MAPbI_3$. For the NVT simulations, eight independent simulation cells were used, with the shaded area representing the range between minimum and maximum values. The solid lines depict the free energy computed for the average NPT MD simulation cell at the temperature that is closest to the given x-axis value on a logarithmic scale. The arrows originating from the solid lines represent corrections to the free energy plotted above, while the arrows pointing toward the solid lines represent corrections arising from the free energy plotted below.

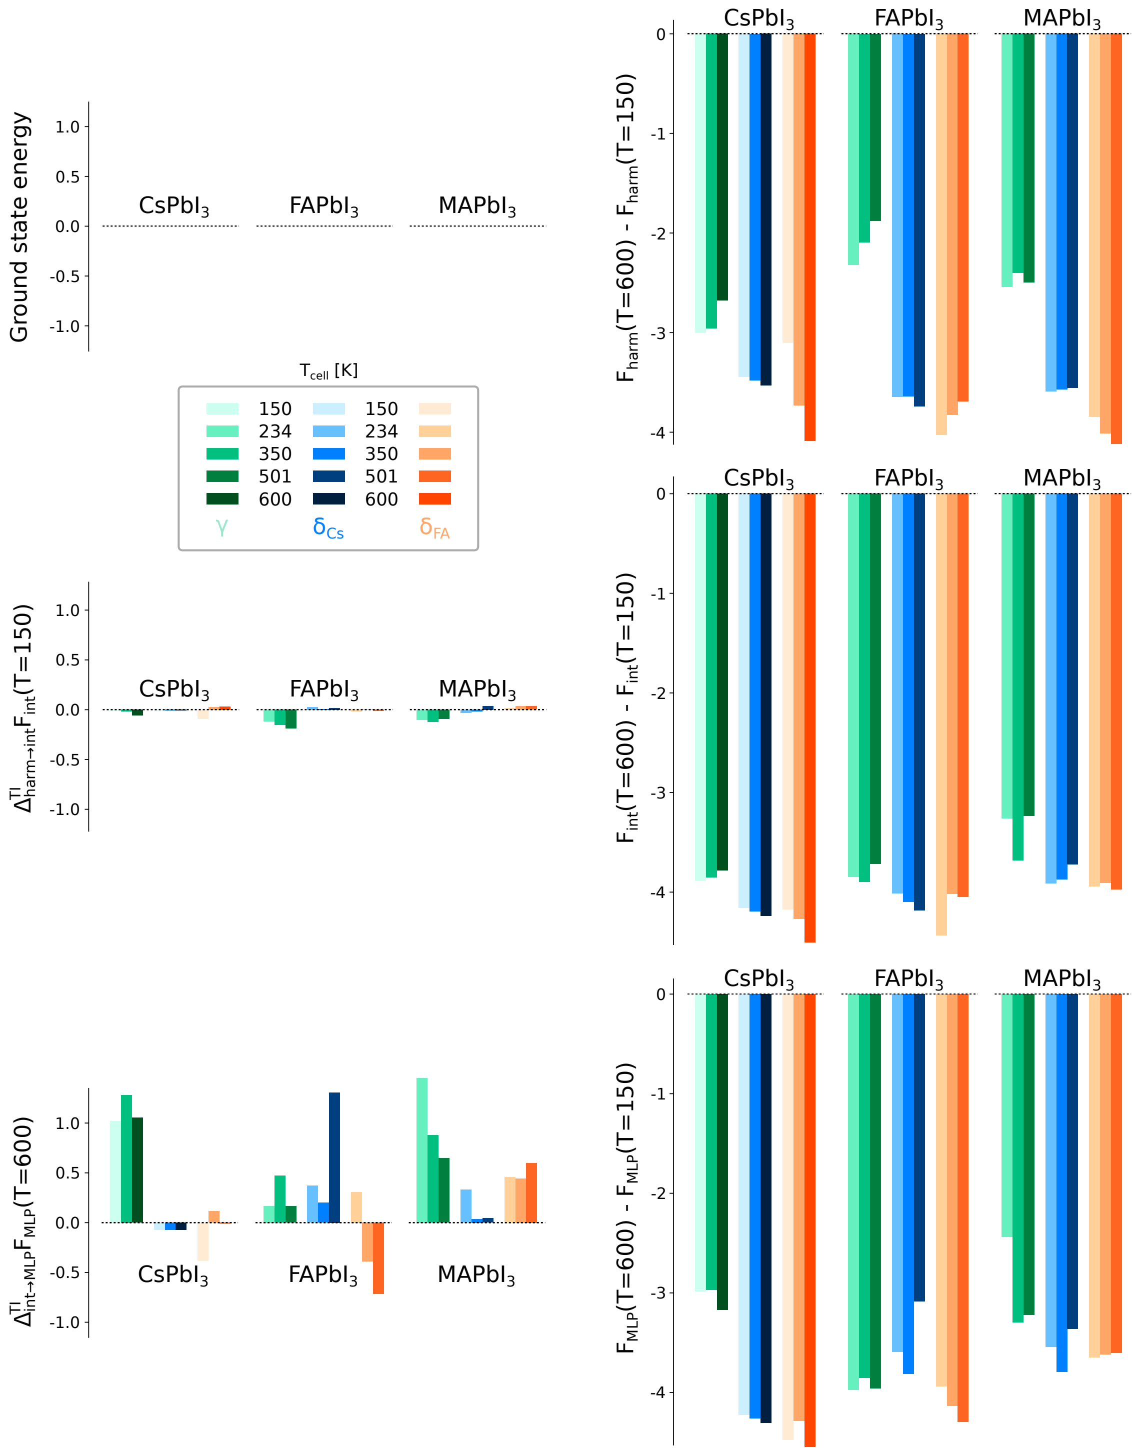


Figure S22: Free energy contributions to the total Helmholtz free energies calculated with the average simulation cells at three different temperatures, see Eq. 2.8 in the manuscript. The energy differences between the contributions for 64 and 8 formula units are reported, positive values indicate that the phase is more stable for 8 formula units. The results of the three phases of $CsPbI_3$, $FAPbI_3$, and $MAPbI_3$ are shown. The left side shows the ground state energy and the $\lambda$-TI corrections to the intermediate and MLP PES. The right side indicates the temperature effect on the free energy for the harmonic, intermediate, and MLP PES.

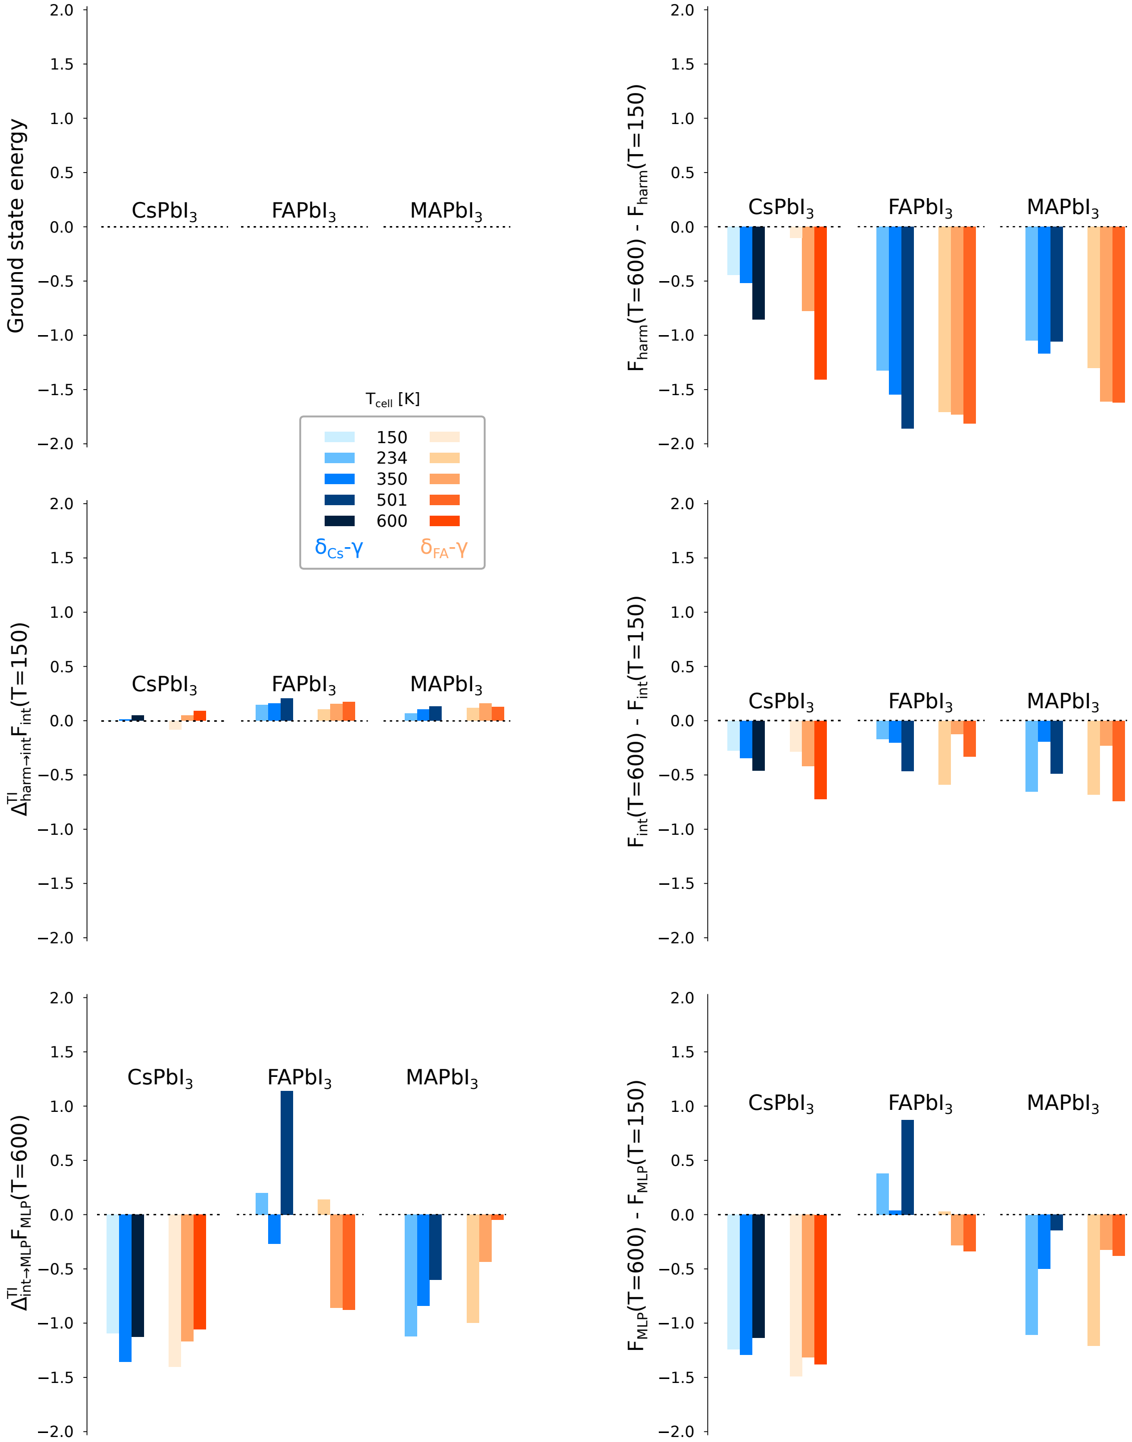


Figure S23: Free energy contributions to the total Helmholtz free energies calculated with the average simulation cells at three different temperatures, see Eq. 2.8 in the manuscript. The effect of the supercell on the energy differences of the $\delta$ phases with respect to the $\gamma$ phase is reported. Positive values indicate that the $\gamma$ phase is more stable for simulation cells with 64 formula units instead of 8. The left side shows the ground state energy and the $\lambda$-TI corrections to the intermediate and MLP PES. The right side indicates the temperature effect on the free energy for the harmonic, intermediate, and MLP PES.

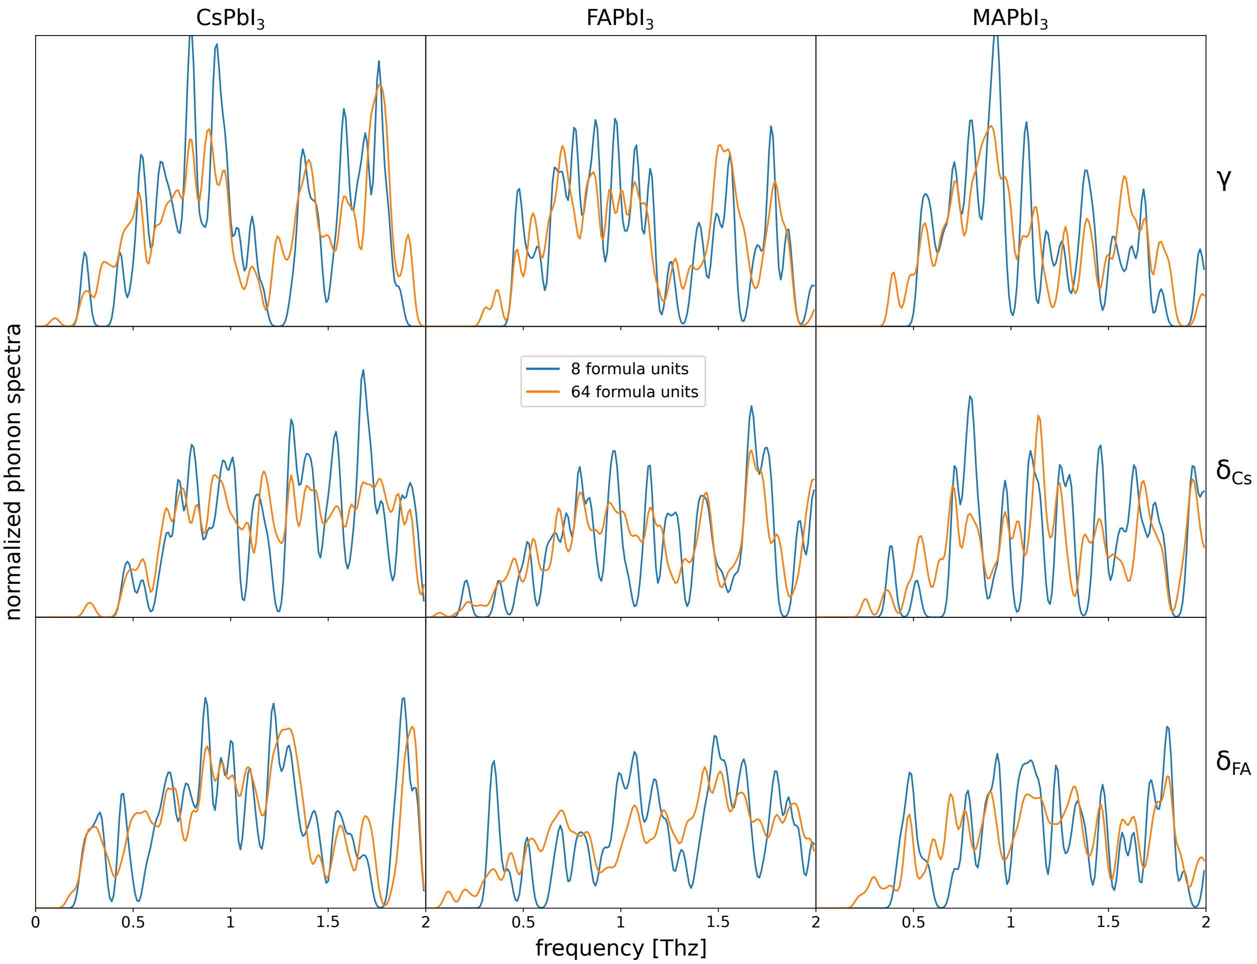


Figure S24: The normalized phonon spectra for the three phases of $CsPbI_3$, $FAPbI_3$, and $MAPbI_3$ for simulations containing 8 and 64 formula units. Calculated via the Hessian matrix of the lowest energy structure that was optimized keeping the simulation cell fixed to the average cell at 350 K and 0.1 MPa. Gaussian smearing of 0.02 THz is added to the eigenvalues of the mass-weighted Hessian.

## 9 Orientation of the organic molecules

Figs. S25 and S26 show the possible orientations of the organic molecules in $FAPbI_3$ and $MAPbI_3$, respectively. The coloring of the dots is based on the orientation of the reference organic molecule, where the RGB values are set by the x, y, and z values of the CN unit vector. For $FAPbI_3$ we can see that the colors mix for the three phases even at the lowest temperature. Similarly for the $MAPbI_3$ phases, the colors mix except for the $\gamma$ phase at 150 K. This means that the orientation of one MA molecule influences the orientation of the other MA molecules reducing the number of local minima that can be sampled at 150 K. At higher temperatures (and for bigger simulation cells, see also Fig. 8 in the manuscript), the organic molecules have more freedom to orient irrespective of neighboring molecules. This may explain why the configurational free energy contribution becomes increasingly stabilizing for the $\gamma$ phase of $MAPbI_3$ at higher temperatures.

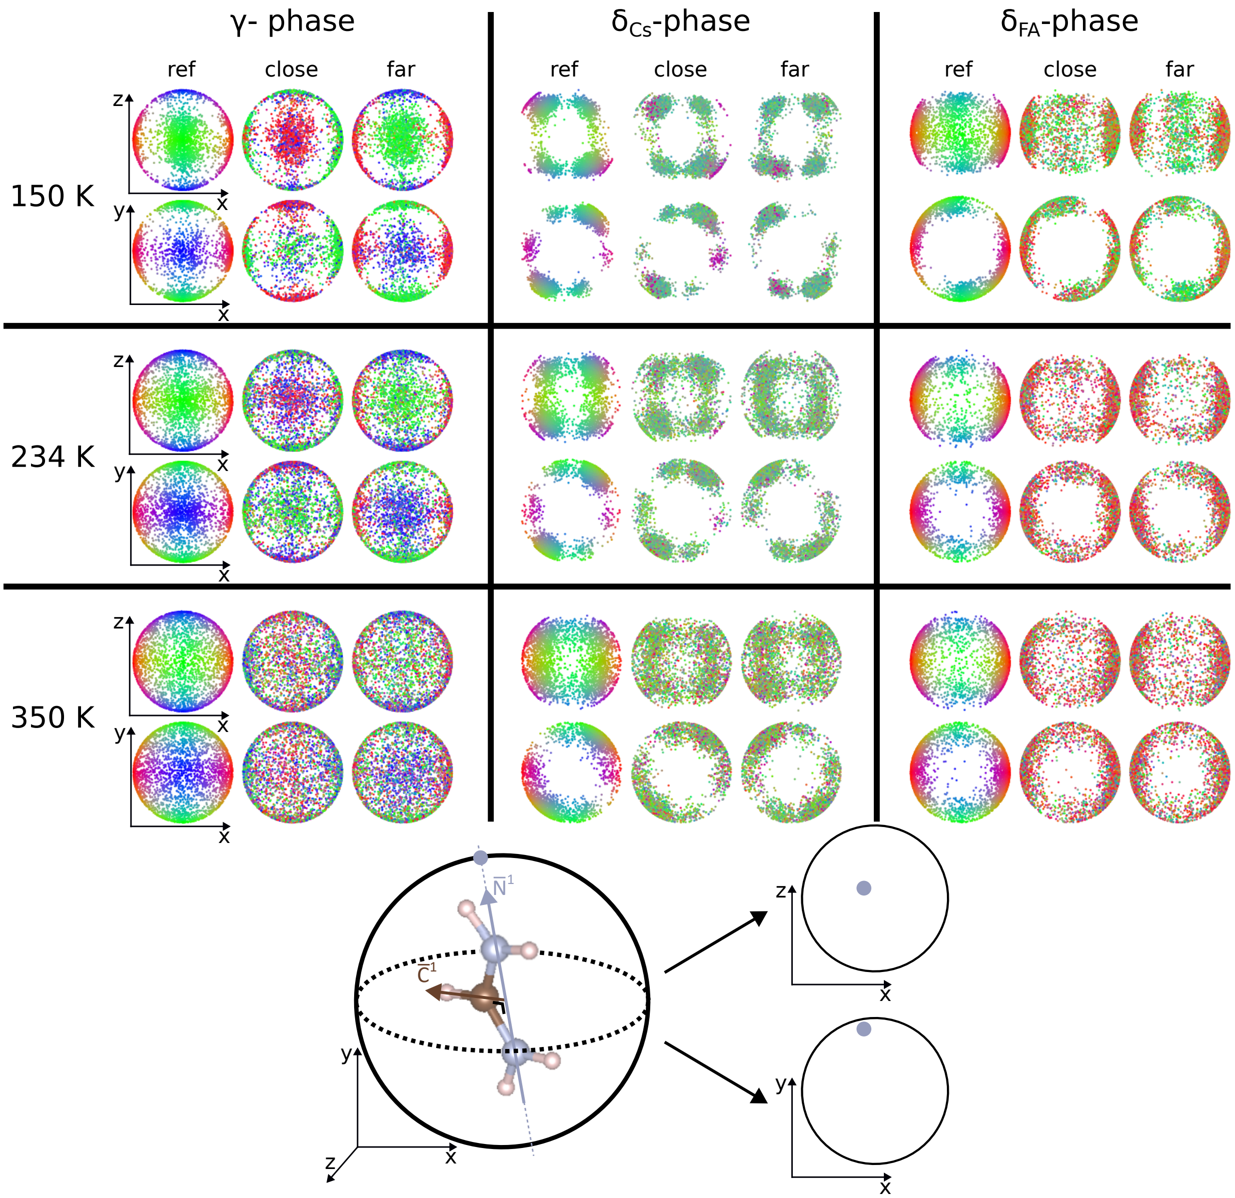


Figure S25: Orientation distributions of three FA molecules in $FAPbI_3$ during NVT simulations on the MLP PES at the specified temperature using the average simulation cell at that temperature. The orientation of each molecule is represented by the unit vector $\overrightarrow{N}$, defined from the two nitrogen atoms. The endpoints of these vectors are projected onto the $xz$ and $xy$ planes, as illustrated at the bottom of the figure. For each simulation, three FA molecules are selected: one is randomly chosen as the reference, and the other two are the nearest and furthest molecules from the reference. The RGB color of each dot is determined by the $x$, $y$, and $z$ components of the $\overrightarrow{N}$ vector of the reference MA molecule in the simulation cell.

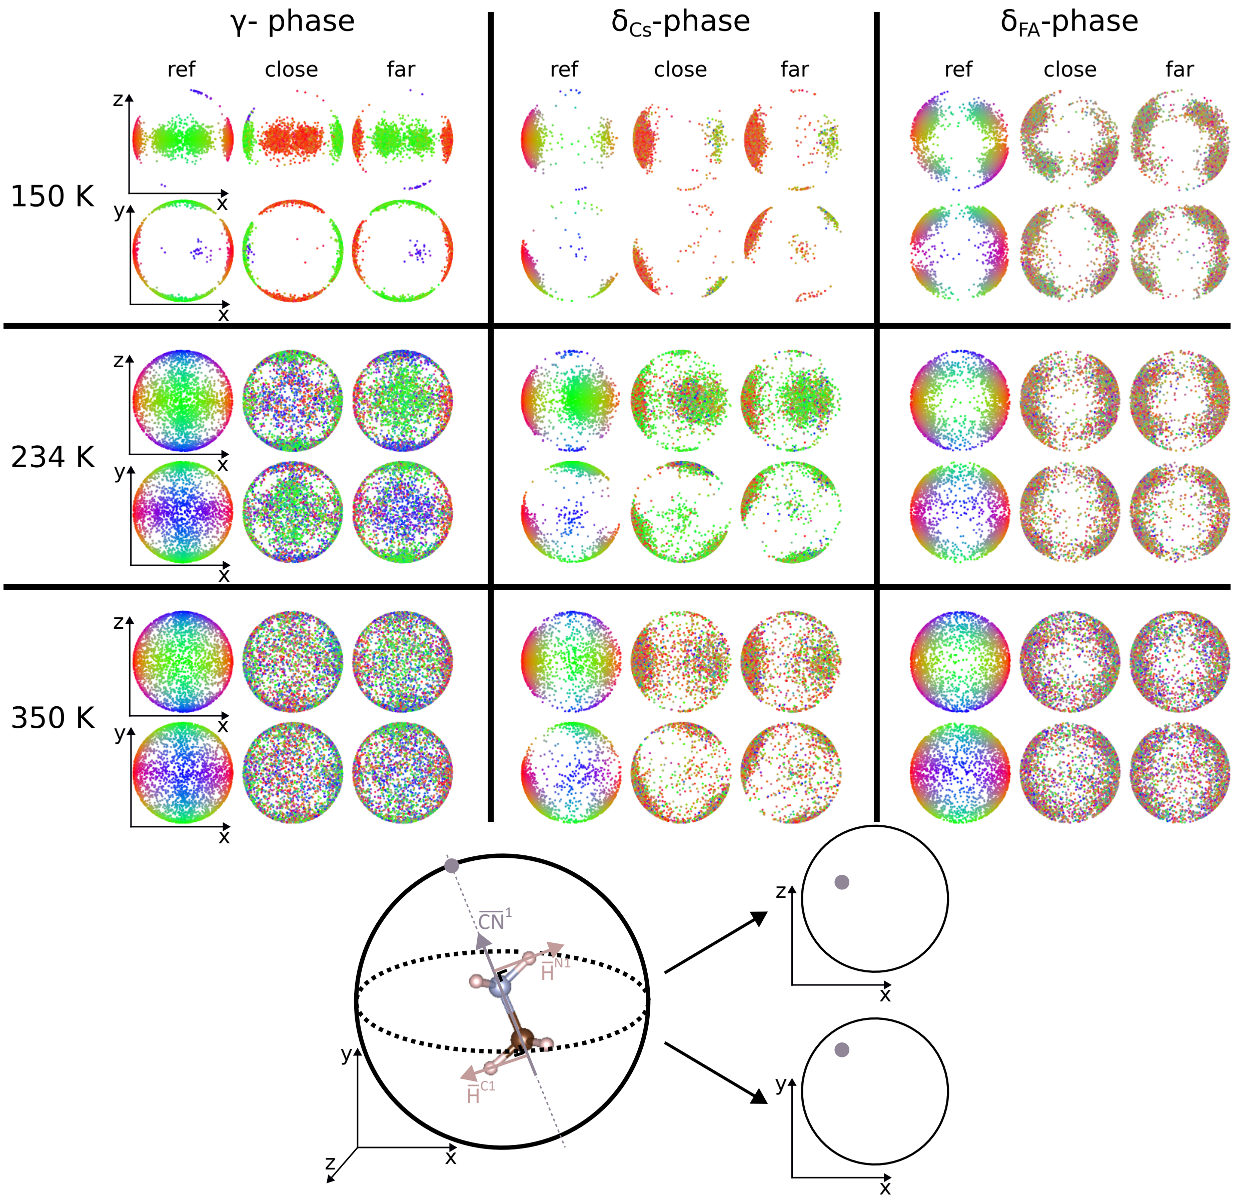


Figure S26: Orientation distributions of three MA molecules in $MAPbI_3$ during NVT simulations on the MLP PES at the specified temperature using the average simulation cell at that temperature. The orientation of each molecule is represented by the unit vector $\overrightarrow{CN}$, defined from the two nitrogen atoms. The endpoints of these vectors are projected onto the $xz$ and $xy$ planes, as illustrated at the bottom of the figure. For each simulation, three MA molecules are selected: one is randomly chosen as the reference, and the other two are the nearest and furthest molecules from the reference. The RGB color of each dot is determined by the $x$, $y$, and $z$ components of the $\overrightarrow{CN}$ vector of the reference MA molecule in the simulation cell.

## References

(1) Peters, L. D. M.; Dietschreit, J. C. B.; Kussmann, J.; Ochsenfeld, C. Calculating free energies from the vibrational density of states function: Validation and critical assessment. *J. Chem. Phys.* **2019**, *150*, 194111.

(2) Kapil, V.; Engel, E.; Rossi, M.; Ceriotti, M. Assessment of Approximate Methods for Anharmonic Free Energies. *Journal of Chemical Theory and Computation* **2019**, *15*, 5845–5857.

(3) Braeckevelt, T.; Goeminne, R.; Vandenhaute, S.; Borgmans, S.; Verstraelen, T.; Steele, J. A.; Roeffaers, M. B. J.; Hofkens, J.; Rogge, S. M. J.; Van Speybroeck, V. Accurately Determining the Phase Transition Temperature of $CsPbI_3$ via Random-Phase Approximation Calculations and Phase-Transferable Machine Learning Potentials. *Chemistry of Materials* **2022**, *34*, 8561–8576.

(4) Beveridge, D. L.; DiCapua, F. M. Free Energy Via Molecular Simulation: Applications to Chemical and Biomolecular Systems. *Annual Review of Biophysics* **1989**, *18*, 431–492.

(5) Cheng, B.; Ceriotti, M. Computing the absolute Gibbs free energy in atomistic simulations: Applications to defects in solids. *Phys. Rev. B* **2018**, *97*, 054102.
